# Supplementary material for: A Differential Entropy Estimator for Training Neural Networks
Source: arXiv:2202.06618 source file (2022-06-19)
Supplement: Supplementary file 1 [file appendix.pdf]

## A Experimental Details of Experiments with Synthetic Data

### A.1 Differential Entropy Estimation of Gaussian Data

In Section 3.1.1, the estimation of the entropy  $h(X) = \frac{d}{2} \log 2\pi e$  for  $X \sim \mathcal{N}(\mathbf{0}, I_d)$  was performed with the hyperparameters given in Table 3. The mean error and its empirical standard deviation are reported over 20 runs, where an independently drawn evaluation set is used that has the same size as the training set.

In the experiment depicted in Figure 1, entropy is decreased after every epoch by letting  $X_i \sim \mathcal{N}(\mathbf{0}, a^i I_d)$ , where  $i = 0, \dots, 4$  is the epoch index. That is,  $X_i = \sqrt{a^i} G^d$ , where  $G$  is a standard normal random variable, resulting in an decrease of the differential entropy by  $\Delta = -\frac{d}{2} \log a \approx 22.18$  for  $a = \frac{1}{2}$  with every epoch. We start at  $h(X_0) = \frac{d}{2} \log 2\pi e \approx 90.81$  and successively decrease until  $h(X_4) = h(X_0) + 4\Delta \approx 2.1$ . Additional parameters can be found in Table 4.

**Computational Resources.** Training was performed on an NVidia V100 GPU. Taken together, training for the first experiments of entropy estimation in dimensions  $d = 10, 64$ , as well as the experiment depicted in Figure 1 used GPU time of less than 5 minutes.

### A.2 Differential Entropy Estimation of Triangle Mixtures

In Section 3.1.2, we perform an estimation of the entropy of  $c$ -component triangle mixture distributions. The pdf of such a  $c$ -component triangle-mixture, is given by

$$p(x) = \sum_{i=1}^c w_i \Lambda_{s_i} \left( x - i - \frac{1}{2} \right), \quad (14)$$

where  $\Lambda_s(x) := \frac{1}{s} \max\{0, 2 - 4s|x|\}$  is a centered triangle pdf with width  $s > 0$ . The scales  $\mathbf{s} = (s_1, \dots, s_c)$  and weights  $\mathbf{w} = (w_1, \dots, w_c)$  satisfy  $0 < s_i, w_i < 1$  and  $\sum_{i=1}^c w_i = 1$ . Before the experiment, we choose  $\mathbf{w}$  uniformly at random from the  $c$ -probability simplex and the scales are chosen uniformly at random in  $[0.1, 1.0]$ . An example for  $c = 10$  is the true pdf depicted in Figure 2 (left). For  $d > 1$ , we perform the estimation on  $d$  i.i.d. copies. Note that the triangle mixture with  $c$  components in  $d$ -dimensional space has  $c^d$  modes, i.e., the support can be partitioned into  $c^d$  disjoint components.

The parameters of the experiment yielding Figure 2 (left) are given in Table 5, while the details of the experiment depicted in Figure 2 (right) can be found in Table 6. The reported accuracy and standard deviation is empirically calculated over all 10 runs, where the evaluation set is independent of the training set and has the same size as the training set.

Table 3: Experimental details of first experiment in Section 3.1.1.

| Parameter               | Value                                 |
|-------------------------|---------------------------------------|
| Source Distribution $X$ | $X \sim \mathcal{N}(\mathbf{0}, I_d)$ |
| Dimension $d$           | 10 and 64                             |
| Optimizer               | Adam [50]                             |
| Learning Rate           | 0.01                                  |
| Batch Size $N$          | 128                                   |
| Kernel Size $M$         | 128                                   |
| Iterations per epoch    | 200                                   |
| Epochs                  | 1                                     |
| Runs                    | 20                                    |

Table 4: Experimental details of the experiment depicted in Figure 1.

| Parameter               | Value                                                              |
|-------------------------|--------------------------------------------------------------------|
| Source Distribution $X$ | $X \sim \mathcal{N}(\mathbf{0}, a^i I_d)$<br>for $i = 0, \dots, 4$ |
| Dimension $d$           | 64                                                                 |
| Factor $a$              | $\frac{1}{2}$                                                      |
| Optimizer               | Adam [50]                                                          |
| Learning Rate           | 0.01                                                               |
| Batch Size $N$          | 128                                                                |
| Kernel Size $M$         | 128                                                                |
| Iterations per epoch    | 1000                                                               |
| Epochs                  | 5                                                                  |
| Runs                    | 1                                                                  |

Table 5: Experimental details of the experiment resulting in the pdf in Figure 2 (left).

| Parameter               | Value                            |
|-------------------------|----------------------------------|
| Source Distribution $X$ | $c$ -component triangle mixtures |
| Components $c$          | 10                               |
| Dimension $d$           | 1                                |
| Optimizer               | Adam [50]                        |
| Learning Rate           | 0.1                              |
| Batch Size $N$          | 128                              |
| Kernel Size $M$         | 128                              |
| Iterations per epoch    | 100                              |
| Epochs                  | 10                               |
| Runs                    | 1                                |

Table 6: Experimental details of the experiment resulting in the training depicted in Figure 2 (right).

| Parameter               | Value                            |
|-------------------------|----------------------------------|
| Source Distribution $X$ | $c$ -component triangle mixtures |
| Components $c$          | 2                                |
| Dimension $d$           | 8                                |
| Optimizer               | Adam [50]                        |
| Learning Rate           | 0.001                            |
| Batch Size $N$          | 128                              |
| Kernel Size $M$         | 128                              |
| Iterations per epoch    | 1000                             |
| Epochs                  | 20                               |
| Runs                    | 10                               |

Table 7: Experimental details of the training depicted in Figure 3 (bottom).

| Parameter            | Value                      |
|----------------------|----------------------------|
| Dimension $d$        | 20                         |
| Optimizer            | Adam [50]                  |
| Learning Rates       | 0.01, 0.003, 0.001, 0.0003 |
| Batch Size $N$       | 128                        |
| Kernel Size $M$      | 128                        |
| Iterations per epoch | 20 000                     |
| Epochs               | 1                          |
| Runs                 | 10                         |

**Computational Resources.** Training was performed on an NVidia V100 GPU. Training in  $d = 1$  dimension, that resulted in Figure 2 (left) can be performed in seconds, while all training required for producing Figure 2 (right) used approximately 1.5 hours of GPU time.

### A.3 Mutual Information Estimation

In Section 3.1.1, we estimate  $I(X^d; Y^d)$  and  $I(X^d; (Y^3)^d)$  where  $(X, Y)$  are multivariate correlated Gaussian distributions. All neural networks are randomly initialized. The bias, variance, and MSE during training, as a function of the MI, can be observed in Figure 5.

In Section 3.2.2, we estimate  $I(X^d; Y^d)$  where  $X, E \sim \mathcal{U}[-\sqrt{3}, \sqrt{3}]$  are independent and  $Y$  is given by  $Y = \rho X + \sqrt{1 - \rho^2} E$  with  $0 < \rho < 1$ . The estimation is performed in 10 runs, randomly choosing the training meta-parameters as proposed by [10]. In Figure 3 (bottom), we present the best run for each method, selected by distance from the true MI at the end of training. The bias, variance, and MSE during training, as a function of the MI, can be observed in Figure 6. Details about the source distribution as well as details of the experiments can be found in Table 7. During experimentation it turned out to be beneficial to train the parameters  $\Theta$  and  $\theta$  in (10) separately and substantially increase the learning rate for the training of  $\theta$ . Thus, we increase the learning rate for the training of  $\theta$  by a factor of  $10^3$ .

**Model Architecture for  $\Theta$ .** We utilize the feed-forward architecture, also used in [10]. It is a simple architecture with two linear layers, one hidden layer using tanh activation, immediately followed by an output layer. The number of neurons in the hidden layer is a meta-parameter selected randomly from  $\{64, 128, 256\}$  for each training run. Three models with this architecture are used for the three parameters  $(\mathbf{A}, \mathbf{a}, \mathbf{u})$ , as described by (6), where only the output dimension is changed to fit the parameter dimension.

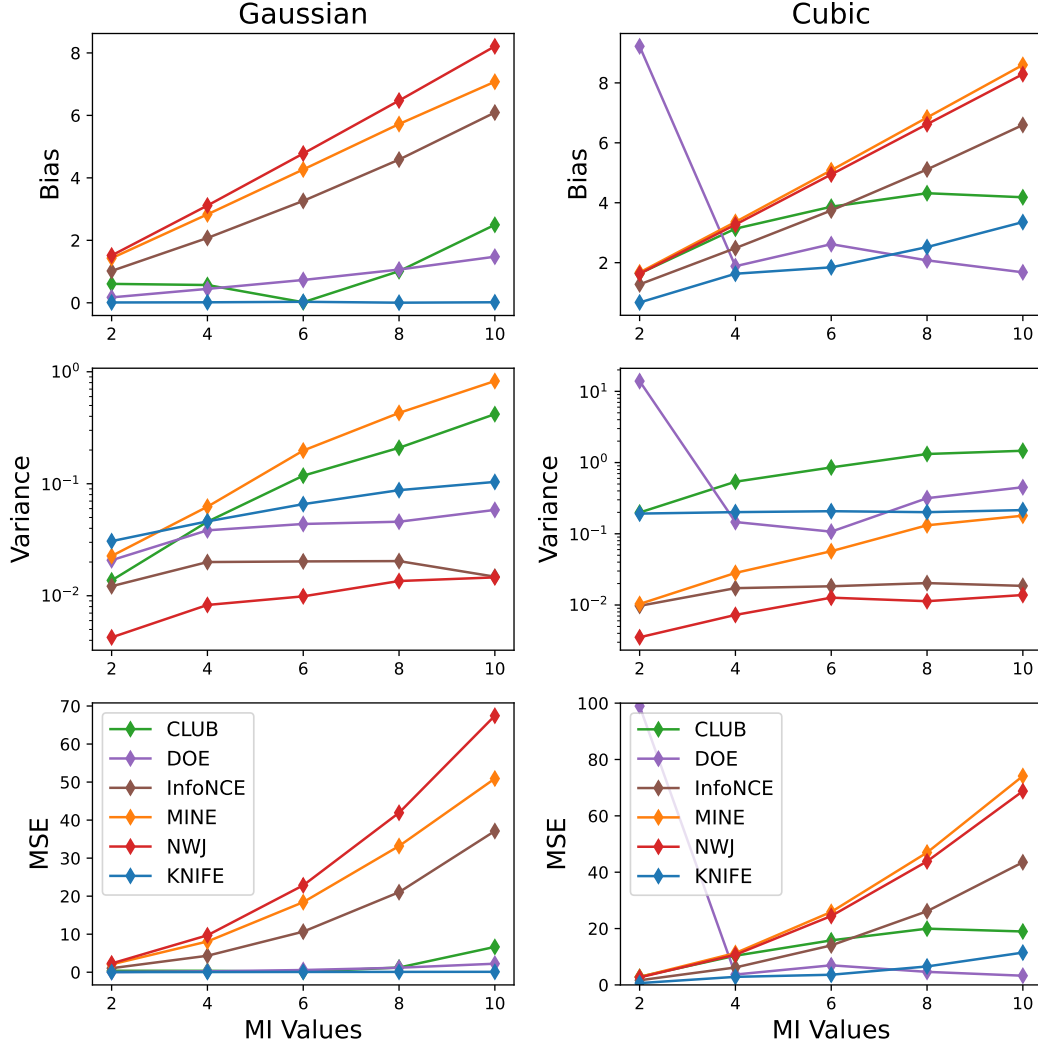

Figure 5: **Left:** Estimation of  $I(X; Y)$ ; **Right:** Estimation of  $I(X; Y^3)$  (cubic transformation).

574 **Computational Resources.** Training was performed, using about 6 hours of GPU time on an  
575 NVidia V100 GPU to carry out the experiment depicted in Figure 3 (bottom).

## 576 B Experimental Details of Experiments on Natural Data

### 577 B.1 Information Bottleneck for Language Model Finetuning

578 For this experiment we follow the experimental setting introduced in [27].<sup>4</sup>

579 **Model Architecture.** We report in Table 8, the multilayer perceptron (MLP) used to compute the  
580 compressed sentence representations produced by BERT. Variance and Mean MLP networks are  
581 composed of fully connected layers.

582 **Model Training.** For model training, all models are trained for 6 epochs and we use early stopping  
583 (best model is selected on validation set error). For IB,  $\lambda$  is selected in  $\{10^{-4}, 10^{-5}, 10^{-6}\}$  and  $K$  is  
584 selected in  $\{144, 192, 288, 384\}$ . We follow [29] where the posterior is averaged over 5 samples and  
585 a linear annealing schedule is used for  $\lambda$ . Additional hyper-parameters are reported in Table 9.

<sup>4</sup>We build on the code provided in <https://githubmemory.com/repo/rabeehk/vibert>.

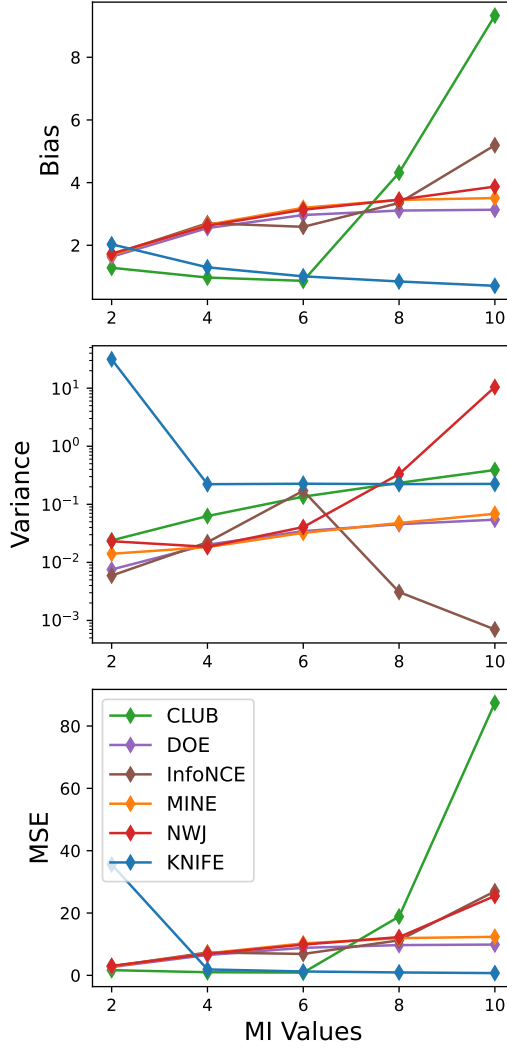

Figure 6: Bias, variance, and MSE for MI estimation on uniformly distributed data.

Table 8: Architecture of the model used in the IB finetuning experiment. We use ReLU as an activation function.

| Layer type      | Input shape        | Output shape       |
|-----------------|--------------------|--------------------|
| Fully connected | 768                | $\frac{2304+K}{4}$ |
| Fully connected | $\frac{2304+K}{4}$ | $\frac{768+K}{2}$  |

Table 9: Experimental details on Information Bottleneck.

| Parameter     | Value                              |
|---------------|------------------------------------|
| Learning Rate | See <a href="#">subsection B.1</a> |
| Optimizer     | AdamW                              |
| Warmup Steps  | 0.0                                |
| Dropout       | 0.0                                |
| Batch Size    | 32                                 |

Table 10: Datasets from the GLUE as used in our experiments.

|       | #Labels        | Train | Val.  | Test |
|-------|----------------|-------|-------|------|
| RTE   | 2              | 2.5k  | 0.08k | 3k   |
| STS-B | 1 (regression) | 5.8k  | 1.5k  | 1.4k |
| MRPC  | 2              | 3.7k  | 0.4k  | 1.7k |

586 **Dataset Statistics.** Table 10 reports the statistics of the dataset used in our finetuning experiment.

587 **Computational Resources.** For all these experiments we rely on NVidia-P100 with 16GB of RAM.  
 588 To complete the full grid-search on 10 seeds and on the three datasets, approximately 1.5k hours are  
 589 required.

## 590 B.2 Fair Textual Classification

591 In this section, we gather the experimental details for the textual fair classification task.

### 592 B.2.1 Details of the KNIFE-based Estimator

593 In this experiment, we estimate the MI between a continuous random variable, namely  $Z = \Phi_\psi(X)$ ,  
 594 and a discrete variable, denoted by  $S \in \mathcal{S} = \{1, 2, \dots, |\mathcal{S}|\}$ . We follow the strategy outlined in  
 595 Section 2.2 for estimating the conditional differential entropy  $h(Z|S)$ . However, we will reuse the  
 596 estimate of the conditional pdf  $\hat{p}(z|s; \Theta)$  to compute an estimate of the differential entropy as

$$h(Z) \approx -\frac{1}{N} \sum_{n=1}^N \log \left( \sum_{s \in \mathcal{S}} \hat{p}_{\text{KNIFE}}(z_n|s; \Theta) \hat{p}(s) \right), \quad (15)$$

597 where  $\hat{p}(s) = \frac{1}{N} |\{n : s_n = s\}|$  is used to indicate the empirical distribution of  $S$  in the training set  
 598  $\mathcal{D}_s$ .<sup>5</sup> In our experiments, with  $|\mathcal{S}| = 2$ , we found that estimating the differential entropy  $h(Z)$  based  
 599 on the KNIFE estimator learnt for  $h(Z|S)$  increases the stability of training.

### 600 B.2.2 Experimental Details

601 **Model Architecture.** For the encoder, we use a bidirectional GRU with two layers with hidden  
 602 and input dimension set to 128. We use LeakyReLU as the activation function. The classification  
 603 head is composed of fully connected layers of input dimension 256. We use a learning rate of 0.0001  
 604 for AdamW. The dropout rate is set to 0.2. The number of warmup steps is set to 1000.

605 **Computational Resources.** For all these experiments, we rely on NVIDIA-P100 with 16GB of  
 606 RAM. Each model is trained for 30k steps. The model with the lowest MI is selected. The training of  
 607 a single network takes around 3 hours.

## 608 B.3 Unsupervised Domain Adaptation

609 We follow the experimental setup given in [30] as closely as possible, i.e., we pick hyperparameters  
 610 given in the paper, or if not provided, those set in the code:<sup>6</sup>

611 **Model Training.** We use Adam optimizer for all modules with a learning rate of 0.001. Batch size  
 612 is set to 128. We set the weighting parameter  $\lambda = 0.1$ . The original code of [30] uses 15 000 training  
 613 iterations, but we found most methods had not properly converged at this stage, and hence use 25 000  
 614 iterations instead. Similar to other experiments, we set the kernel size  $M = 128$ .

615 **Model Architecture.** Table 11 summarizes the architectures used for the different modules. For  
 616 the MI network of each method, the best configuration, based on the validation set of the first task  
 617 MNIST  $\rightarrow$  MNIST-M, is chosen among 4 configurations: with or without LayerNorm and with ReLU  
 618 or tanh activation.

619 **Computational Resources.** For these experiments, we used a cluster of NVIDIA-V100 with 16GB  
 620 of RAM. Each training (i.e., 25k iterations) on a single task requires on average 2 hours. Given that  
 621 we have 6 tasks, and repeat the training for 3 different seeds, on average 36 hours computation time  
 622 is required for each method.

<sup>5</sup>As we work with balanced batches, we will have  $\hat{p}(s) = \frac{1}{|\mathcal{S}|}$ .

<sup>6</sup>[https://github.com/Linear95/CLUB/tree/master/MI\\_DA](https://github.com/Linear95/CLUB/tree/master/MI_DA).

Table 11: Architectures used for the Unsupervised Domain Adaptation experiments. For the MI network of each method, we chose the best performing configuration between with or without LayerNorm layer and best activation between ReLU and tanh, using the validation set of MNIST-M.

| <b>Encoder (both <math>\Phi</math> and <math>\Phi^d</math>)</b> |                      |                      |           |  |  |
|-----------------------------------------------------------------|----------------------|----------------------|-----------|--|--|
| Layer type                                                      | Input shape          | Output shape         | Details   |  |  |
| Convolution sequence                                            | (3, H, W)            | (64, H, W)           | Cf. below |  |  |
| Noisy downsampling                                              | (64, H, W)           | (64, H // 2, W // 2) | Cf. below |  |  |
| Convolution sequence                                            | (64, H // 2, W // 2) | (64, H // 2, W // 2) | Cf. below |  |  |
| Noisy downsampling                                              | (64, H // 2, W // 2) | (64, H // 4, W // 4) | Cf. below |  |  |
| Convolution sequence                                            | (64, H // 4, W // 4) | (64, H // 4, W // 4) | Cf. below |  |  |
| Global Average Pool                                             | (64, H // 4, W // 4) | (64,)                | -         |  |  |

  

| <b>Main classifier <math>C</math></b> |             |              | <b>Domain classifier <math>C^d</math></b> |             |              |
|---------------------------------------|-------------|--------------|-------------------------------------------|-------------|--------------|
| Layer type                            | Input shape | Output shape | Layer type                                | Input shape | Output shape |
| Fully connected                       | (64,)       | (10,)        | Fully connected                           | (64,)       | (2,)         |

  

| <b>Convolution sequence</b> |             |              |                                       |
|-----------------------------|-------------|--------------|---------------------------------------|
| Layer type                  | Input shape | Output shape | Parameters                            |
| 2D convolution              | (3, H, W)   | (64, H, W)   | 3x3, 64 channels, Stride=1, Padding=1 |
| 2D BatchNorm                | (3, H, W)   | (64, H, W)   | -                                     |
| Activation                  | (3, H, W)   | (64, H, W)   | LeakyRelu 0.1                         |
| 2D convolution              | (64, H, W)  | (64, H, W)   | 3x3, 64 channels, Stride=1, Padding=1 |
| 2D BatchNorm                | (64, H, W)  | (64, H, W)   | -                                     |
| Activation                  | (64, H, W)  | (64, H, W)   | LeakyRelu 0.1                         |
| 2D convolution              | (64, H, W)  | (64, H, W)   | 3x3, 64 channels, Stride=1, Padding=1 |
| 2D BatchNorm                | (64, H, W)  | (64, H, W)   | -                                     |
| Activation                  | (64, H, W)  | (64, H, W)   | LeakyRelu 0.1                         |

  

| <b>Noisy downsampling</b> |                      |                      |                            |
|---------------------------|----------------------|----------------------|----------------------------|
| Layer type                | Input shape          | Output shape         | Parameters                 |
| MaxPool                   | (64, H, W)           | (64, H // 2, H // 2) | 2x2, Stride=2              |
| Dropout                   | (64, H // 2, W // 2) | (64, H // 2, H // 2) | p=0.5                      |
| Noise                     | (64, H // 2, W // 2) | (64, H // 2, H // 2) | Gaussian with $\sigma = 1$ |

  

| <b>MI network</b> |               |                |                           |
|-------------------|---------------|----------------|---------------------------|
| Layer type        | Input shape   | Output shape   | Details                   |
| LayerNorm         | ( $C_{in,}$ ) | ( $C_{in,}$ )  | Optional                  |
| Fully connected   | ( $C_{in,}$ ) | (64,)          | Activation = [ReLU, tanh] |
| LayerNorm         | ( $C_{in,}$ ) | (64,)          |                           |
| Fully connected   | (64,)         | ( $C_{out,}$ ) | Optional                  |
