# Supplementary material for: A Differential Entropy Estimator for Training Neural Networks
Source: arXiv:2202.06618 source file (2022-06-19)
Supplement: Supplementary file 3 [file submission_with_appendix2.pdf]

---

# KNIFE: Kernelized-Neural Differential Entropy Estimation

---

Anonymous Author(s)

Affiliation

Address

email

## Abstract

1 Estimation of mutual information has been pursued with significant efforts by  
2 the machine learning community. However, the estimation of the closely related  
3 differential entropy did hardly receive any attention in the last decades. In this  
4 paper, we introduce KNIFE, a fully parameterized, differentiable kernel-based  
5 estimator of differential entropy. The flexibility of our approach allows us to  
6 construct KNIFE-based estimators for conditional (on either discrete or continuous  
7 variables) differential entropy, as well as mutual information. We empirically  
8 validate these estimators on high-dimensional synthetic data and further apply them  
9 to guide the training of neural networks for real-world tasks. Our experiments on a  
10 large variety of tasks, including visual domain adaptation, textual fair classification,  
11 and textual fine-tuning demonstrate the effectiveness of KNIFE-based estimators.

## 12 1 Introduction

13 Entropy and conditional entropy have been extraordinarily valuable in the design of modern com-  
14 munication systems [1] and their use has been recently gaining momentum within the machine  
15 learning (ML) community. Here, they help to specify the design of objectives for training modern ML  
16 models [2, 3]. For instance, entropy has become very popular in reinforcement learning [4, 5, 6, 7],  
17 where entropy maximization is used to encourage exploration and thus, to avoid convergence to poor  
18 low entropy policies.

19 Quantifying the dependence between two continuous or discrete/continuous random variables (e.g.,  
20 concepts and features) is a fundamental ingredient in representation learning, and thus many measures  
21 have been proposed. As a fundamental measure of dependence, Mutual Information (MI) has  
22 been commonly applied in statistics and machine learning to quantify the dependence between  
23 variables. MI has the advantage of providing a very powerful measure of nonlinear associations, e.g.,  
24 compared to Pearson’s correlation coefficient which can only measure linear dependence. As MI  
25 typically cannot be estimated directly [8, 9, 10], estimates of surrogate functions, either upper/lower  
26 bounds [11, 12], are commonly used in place. Recently, there has been a revival of methods inspired  
27 by the celebrated *InfoMax principle* [13], which explore various estimators of upper/lower bounds  
28 of MI that have demonstrated promising empirical results in unsupervised representation learning  
29 [14, 15, 16, 17, 18, 19, 20], discrete/invariant representations [21, 22], generative modelling [23, 24],  
30 textual disentangling [25, 26], applications of the information bottleneck [27, 28, 29], among others.

31 In this paper, we investigate the problem of estimating differential entropy and conditional differential  
32 entropy—fundamental concepts that began as an attempt by Shannon to extend the notion of entropy  
33 to continuous probability distributions—using a finite number of samples. More specifically, given  
34  $N$  i.i.d. samples of a random variable with unknown probability density function (pdf)  $p$ , we propose

35 a fully differentiable kernel-based estimator of the differential entropy:<sup>1</sup>

$$h(X) := - \int p(x) \log p(x) dx. \quad (1)$$

36 MI is intimately linked to differential and conditional differential entropy by noticing that

$$I(X; Y) = h(X) - h(X|Y). \quad (2)$$

37 Although the study of efficient neural-based estimators of MI has undoubtedly played an important  
38 role in the recent development of the field of machine learning (e.g., adversarial and representation  
39 learning), conditional and differential entropy hardly received any attention in recent years.

## 40 1.1 Contributions

41 Our work advances the state-of-the-art methods in differential entropy and MI estimation in several  
42 different ways.

- 43 • We introduce KNIFE, a fully learnable kernel-based estimator of differential entropy. The  
44 parameters of the KNIFE estimator are learned by SGD-optimization of both shape and  
45 multi-modes (e.g., mixing weights, shifts, and covariance matrices). Additionally, KNIFE  
46 does not require distributional assumptions (other than smoothness).
- 47 • The flexibility of our approach allows us to also construct a KNIFE-based estimator for  
48 conditional differential entropy, conditioning on either a discrete or continuous random  
49 variable. This in turn enables us to estimate MI between either two continuous or one  
50 discrete and one continuous random variable.
- 51 • Experiments on various synthetic datasets (including Gaussian, non-Gaussian, and even  
52 multi-modal distributions) clearly show that KNIFE outperforms state-of-the-art methods  
53 on both differential entropy and MI estimation. Indeed, a key ingredient of KNIFE is its  
54 inherent ability to rapidly adapt to changes in the underlying data distribution. According to  
55 our experiments on natural datasets, this feature provides KNIFE with a clear advantage for  
56 representation learning tasks.
- 57 • We conduct experiments on natural datasets (including text and images) to compare KNIFE-  
58 based MI estimators to most recent MI estimators, namely, CLUB [30], InfoNCE [16],  
59 MINE [31], and NWJ [32]. First, we apply KNIFE to the Information Bottleneck (IB)  
60 principle to fine-tune a pretrained language model. There, we are able to leverage the  
61 available closed form of the conditional differential entropy and by only estimating the  
62 differential entropy with KNIFE, we achieve better scores than competing MI estimators.  
63 Second, on a fair textual classification task, the KNIFE-based MI estimator is shown to  
64 achieve near perfect disentanglement (with respect to the private, discrete label) at virtually  
65 no degradation of the accuracy of the main task. Lastly, in the challenging scenario of visual  
66 domain adaptation, where both variables are continuous, KNIFE-based MI estimation is also  
67 able to achieve superior results compared to other recent MI estimators.

## 68 1.2 Existent methods and related works

69 Existing methods for estimating differential entropy fit into one of the three categories [33, 34, 35]:  
70 plug-in estimates [36, 37], estimates based on sample-spacings [38], and estimates based on nearest  
71 neighbor distances [39, 40]. Our proposed estimator falls into the first category and we will thus focus  
72 here on previous work using that methodology. Excellent summaries of all the available methods can  
73 be found in the works [33, 34, 41, 35].

74 In [36], a nonparametric estimator of differential entropy has first been suggested and theoretically  
75 analyzed. It builds on the idea of kernel density estimation using Parzen-Rosenblatt windowing  
76 [42, 43]. More detailed analysis followed [44, 45] but the estimators stayed essentially unchanged.  
77 Unfortunately, this classical literature is mostly concerned with appropriate regularity conditions that  
78 guarantee asymptotic properties of estimators, such as (asymptotic) unbiasedness and consistency. In  
79 machine learning applications, however, it is infeasible to assume that such an estimator operates in

---

<sup>1</sup>All logarithms in this work are to base  $e$  and thus, corresponding information-theoretic quantities are measured in nat.

80 “high sample” regime that justifies the use of asymptotic results. A first estimator that employed a  
 81 differential learning rule was introduced in [46]. Indeed, the estimator proposed therein is already  
 82 optimized using stochastic optimization but due to the limitations of the time only uses a low number  
 83 of parameters, in particular, a single kernel function is learned for all samples. An extension that uses  
 84 a *heteroscedastic* kernel density estimate, i.e., using different kernels at different positions, has been  
 85 proposed in [47]. Still the number of parameters was quite low and a shift in the kernels or variable  
 86 weights were not considered. Although the estimation of differential entropy remained a topic of  
 87 major interest as illustrated by recent works focusing on special classes of distributions [48, 49], the  
 88 estimator introduced in [47] was not further refined and hardly explored in recent works.

89 In contrast, there has been a recent surge on new methods for the estimation of the closely related MI  
 90 between two random variables. The most prominent examples include unnormalized energy-based  
 91 variational lower bounds [11], the lower bounds developed in [32] using variational characterization  
 92 of f-divergence, the MINE-estimator developed in [31] from the Donsker-Varadhan representation of  
 93 MI, the noise-contrastive based bound developed in [16] and finally a contrastive upper bound [30].

## 94 2 KNIFE Estimator

### 95 2.1 Differential entropy

96 **Estimation step:** Consider a continuous random variable  $X \sim p$ . Our goal is to estimate the  
 97 differential entropy  $h(X)$ , as defined in (1). Given the intractability of this integral, we will rely on a  
 98 Monte-Carlo estimate of  $h(X)$ , using  $N$  i.i.d. samples  $\mathcal{D}_x = \{x_n\}_{n=1}^N$  to obtain

$$\hat{h}_{\text{ORACLE}}(\mathcal{D}_x) := -\frac{1}{N} \sum_{n=1}^N \log p(x_n). \quad (3)$$

99 Unfortunately, assuming access to the true density  $p$  is often unrealistic, and we will instead construct  
 100 an estimate  $\tilde{p}$  that can then be plugged into (3) instead of  $p$ .

101 Assuming access to an additional—ideally independent—set of  $M$  i.i.d. samples  $\mathcal{E} = \{x'_m\}_{m=1}^M$ , we  
 102 build upon the Parzen-Rosenblatt estimator [42, 43]

$$\tilde{p}(x; w, \mathcal{E}) = \frac{1}{M} \sum_{m=1}^M \kappa_w(x - x'_m), \quad (4)$$

103 where  $\kappa_w$  is a kernel density with bandwidth  $w > 0$ . The resulting entropy estimator when replacing  
 104  $p$  in (3) by (4) was analyzed in [36]. In [47], this approach was generalized using the kernel estimator  
 105

$$\hat{p}_{\text{Schrau.}}(x; \mathbf{A}, \mathcal{E}) := \frac{1}{M} \sum_{m=1}^M \kappa_{A_m}(x - x'_m), \quad (5)$$

106 where  $\mathbf{A} := (A_1, \dots, A_M)$  are (distinct) covariance matrices and  $\kappa_A = \mathcal{N}(0, A)$  is a centered  
 107 Gaussian density with covariance matrix  $A$ . Our density estimator is an augmentation

$$\hat{p}_{\text{KNIFE}}(x; \boldsymbol{\theta}) := \sum_{m=1}^M u_m \kappa_{A_m}(x - a_m), \quad (6)$$

108 where  $\boldsymbol{\theta} := (\mathbf{A}, \mathbf{a}, \mathbf{u})$  and the additional parameters  $0 \leq \mathbf{u} = (u_1, u_2, \dots, u_M)$  with  $\mathbf{1} \cdot \mathbf{u} = 1$  and  
 109  $\mathbf{a} = (a_1, \dots, a_M)$  are introduced. Note that  $\hat{p}_{\text{KNIFE}}(x; \boldsymbol{\theta})$  is a smooth function of  $\boldsymbol{\theta}$ , and so is our  
 110 proposed plug-in estimator

$$\hat{h}_{\text{KNIFE}}(\mathcal{D}_x; \boldsymbol{\theta}) := -\frac{1}{N} \sum_{n=1}^N \log \hat{p}_{\text{KNIFE}}(x_n; \boldsymbol{\theta}). \quad (7)$$

111 As we will see in synthetic experiments, incorporating  $u_m$  and shifts  $a_m$  in the optimization enables  
 112 the use of KNIFE in a non-stationary settings, where the distribution of  $X$  evolves over time.

113 **Learning step:** Stemming from the observation that, by the Law of Large Numbers (LLN),

$$\hat{h}_{\text{KNIFE}}(\mathcal{D}_x, \theta) \stackrel{\text{LLN}}{\approx} -\mathbb{E} [\log \hat{p}_{\text{KNIFE}}(X; \theta)] = h(X) + D_{\text{KL}}(p \| \hat{p}_{\text{KNIFE}}(\cdot; \theta)) \geq h(X), \quad (8)$$

114 we propose to learn the parameters  $\theta$  by minimizing  $\hat{h}_{\text{KNIFE}}$ , where  $\mathcal{E}$  may be used to initialize  $\theta$ .  
 115 Although not strictly equivalent due to the Monte-Carlo approximation, minimizing  $\hat{h}_{\text{KNIFE}}$  can be  
 116 understood as minimizing the Kullback-Leibler (KL) divergence in (8), effectively minimizing the gap  
 117 between  $\hat{h}_{\text{KNIFE}}$  and  $h(X)$ . In fact,  $\hat{h}_{\text{KNIFE}}$  can also be interpreted as the standard maximum likelihood  
 118 objective, widely used in modern machine learning. It is worth to mention that the KNIFE estimator  
 119 is fully differentiable with respect to  $\theta$  and the optimization can be tackled by any gradient-based  
 120 method (e.g., in our experiment we use Adam [50] or AdamW [51]).

## 121 2.2 Estimating Conditional Differential Entropy and Mutual Information

122 The proposed differential entropy estimator can be used as a building block to estimate other  
 123 information measures. In particular, we can use KNIFE to construct estimators of conditional  
 124 differential entropy and MI. When estimating the conditional differential entropy and MI for a pair of  
 125 random variables  $(X, Y) \sim p$ , we not only use  $\mathcal{D}_x = \{x_n\}_{n=1}^N$ , but also the according i.i.d. samples  
 126  $\mathcal{D}_y = \{y_n\}_{n=1}^N$ , where  $(x_n, y_n)$  are drawn according to  $p$ .

127 **Extension to conditional differential entropy:** We estimate conditional differential entropy  
 128  $h(X|Y)$  by considering  $\theta$  to be a parameterized function  $\Theta(y)$  of  $y$ . Then all relations previously  
 129 established naturally generalize and we write

$$\hat{p}_{\text{KNIFE}}(x|y; \Theta) := \hat{p}_{\text{KNIFE}}(x; \Theta(y)), \quad \hat{h}_{\text{KNIFE}}(\mathcal{D}_x | \mathcal{D}_y; \Theta) := -\frac{1}{N} \sum_{n=1}^N \log \hat{p}_{\text{KNIFE}}(x_n | y_n; \Theta). \quad (9)$$

130 Naturally, minimization of (8) is now performed over the parameters of  $\Theta$ . If  $Y$  is a continuous  
 131 random variable, we use an artificial neural network  $\Theta(y)$ , taking  $y$  as its input. On the other hand, if  
 132  $Y \in \mathcal{Y}$  is a discrete random variable, we have one parameter  $\theta$  for each  $y \in \mathcal{Y}$ , i.e.,  $\Theta = \{\theta_y\}_{y \in \mathcal{Y}}$   
 133 and  $\hat{p}_{\text{KNIFE}}(x|y; \Theta) = \hat{p}_{\text{KNIFE}}(x; \Theta(y)) = \hat{p}_{\text{KNIFE}}(x; \theta_y)$ .

134 **Extension to the mutual information:** To estimate the MI between random variables  $X$  and  
 135  $Y$  (either discrete or continuous), recall that MI can be written as  $I(X; Y) = h(X) - h(X|Y)$ .  
 136 Therefore, we use the marginal and conditional differential entropy estimators (7) and (9) to build a  
 137 KNIFE-based MI estimator as follows

$$\hat{I}_{\text{KNIFE}}(\mathcal{D}_x, \mathcal{D}_y; \theta, \Theta) := \hat{h}_{\text{KNIFE}}(\mathcal{D}_x; \theta) - \hat{h}_{\text{KNIFE}}(\mathcal{D}_x | \mathcal{D}_y; \Theta). \quad (10)$$

## 138 3 Experiments using Synthetic Data

### 139 3.1 Differential Entropy Estimation

140 In this section we apply KNIFE for differential entropy estimation, comparing it to (5), the method  
 141 introduced in [47], subsequently labeled “Schrau.”. We did not perform the Expectation Maximization  
 142 algorithm, as suggested in [47], but instead opted to use the same optimization technique as for  
 143 KNIFE to facilitate a fair comparison. Details regarding the experimental setups can be found in the  
 144 supplementary material.

#### 145 3.1.1 Gaussian Distribution

146 As a sanity check, we test KNIFE on multivariate normal data in moderately high dimensions and  
 147 compare it to (5), which we trained with the exact same parameters.

148 At  $d = 10$  we have the entropy  $h = \frac{d}{2} \log 2\pi e = 14.19$  and an estimation accuracy of  $|h - \hat{h}_{\text{KNIFE}}| \approx$   
 149  $0.0501 \pm 0.0149$ , while  $|h - \hat{h}_{\text{Schrau}}| \approx 0.7493 \pm 0.0525$ . For a higher dimension,  $d = 64$  we  
 150 find  $h = 90.81$  and the bias increases accordingly to  $|h - \hat{h}_{\text{KNIFE}}| \approx 2.6959 \pm 0.0645$ , while  
 151  $|h - \hat{h}_{\text{Schrau}}| \approx 9.9014 \pm 0.2327$ .

In order to use a differential entropy estimation primitive in a machine learning system, it must be able to adapt to a changing input distribution during training. This results in a severe limitation of (5), as re-drawing the kernel support  $\mathcal{E}$  can be either impractical or at the very least requires a complete re-training of the entropy estimator. Whereas in (6), the kernel support  $\mathbf{a}$  is trainable and it can thus adapt to a change of the input distribution. In order to showcase this ability, we utilize the approach of [30] and successively decrease the entropy, observing how the estimator adapts. We perform this experiment with data of dimension  $d = 64$  and repeatedly multiply the covariance matrix of the training vectors with a factor of  $a = \frac{1}{2}$ . The resulting entropy estimation is depicted in Figure 1. It is apparent that (5) suffers from a varying bias. The bias increases with decreasing variance, as the kernel support is fixed and cannot adapt as the variance of  $\mathcal{D}_x$  shrinks.

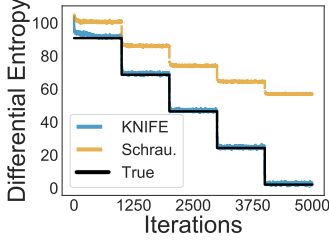

Figure 1: Estimating differential entropy of Gaussian data with  $a = \frac{1}{2}$ .

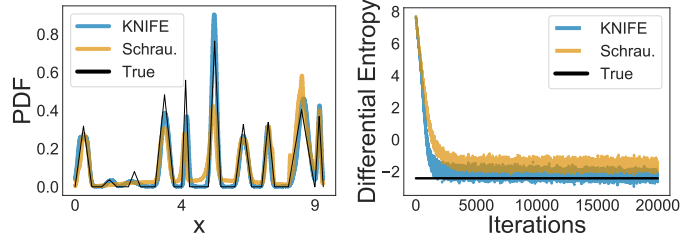

Figure 2: **Left:** PDF when estimating differential entropy of a triangle mixture in 1 dimension. **Right:** Training run when estimating differential entropy of a 2-component triangle mixture in 8 dimensions.

161

### 162 3.1.2 Triangle Mixture

KNIFE is able to cope with distributions that have multiple modes. We illustrate this by matching a mixture of randomly drawn triangle distributions. The resulting estimated pdfs as well as the ground truth when estimating the entropy of a 1-dimensional mixture of triangles with 10 components can be observed in Figure 2 (left). With increasing dimension the difficulty of this estimation rises quickly as in  $d$  dimensions, the resulting pdf of  $c$ -component triangle mixtures has  $c^d$  modes. To showcase the performance of KNIFE in this challenging task, we ran 10 training runs for differential entropy estimation of 2-component triangle mixtures in 8 dimensions. An example training run is depicted in Figure 2 (right). Over ten runs, entropy was estimated to an accuracy of  $0.9286 \pm 0.5697$  by KNIFE and accurate to  $1.5532 \pm 0.5505$  using (5).

## 172 3.2 MI Estimation

### 173 3.2.1 Multivariate Gauss

We repeat the experiments in [30], stepping up the MI  $I(X^d; Y^d)$  between  $d$  i.i.d. copies of joint normal random variables  $(X, Y)$  by increasing their correlation coefficient, i.e.,  $(X, Y)$  are multivariate Gaussian with correlation coefficient  $\rho_i$  in the  $i$ -th epoch. A training run is depicted in the top of Figure 3. As in [30], we also repeat the experiment, applying a cubic transformation to  $Y$ . The estimation of MI between  $d$  i.i.d. copies of  $X$  and  $Y^3$  can be observed in the middle row of Figure 3. The MI is unaffected by this bijective transformation. In the supplementary material, the bias and variance are depicted separately.

### 181 3.2.2 Sum of Uniformly Distributed Variables

In order to test the ability of KNIFE in adapting to distributions, substantially different from the Gaussian kernel shape, we apply it in MI estimation of  $I(X^d; Y^d)$  with uniformly distributed data. To this end, let  $X$  and  $E$  be centered, uniformly distributed random variables with  $\mathbb{E}[X^2] = \mathbb{E}[E^2] = 1$  and define  $Y = \rho_i X + \sqrt{1 - \rho_i^2} E$  in the  $i$ -th epoch. One training run with  $d = 20$  is shown in Figure 3 (bottom). Details about the source distribution as well as details of the experiments can be found in the supplementary material.

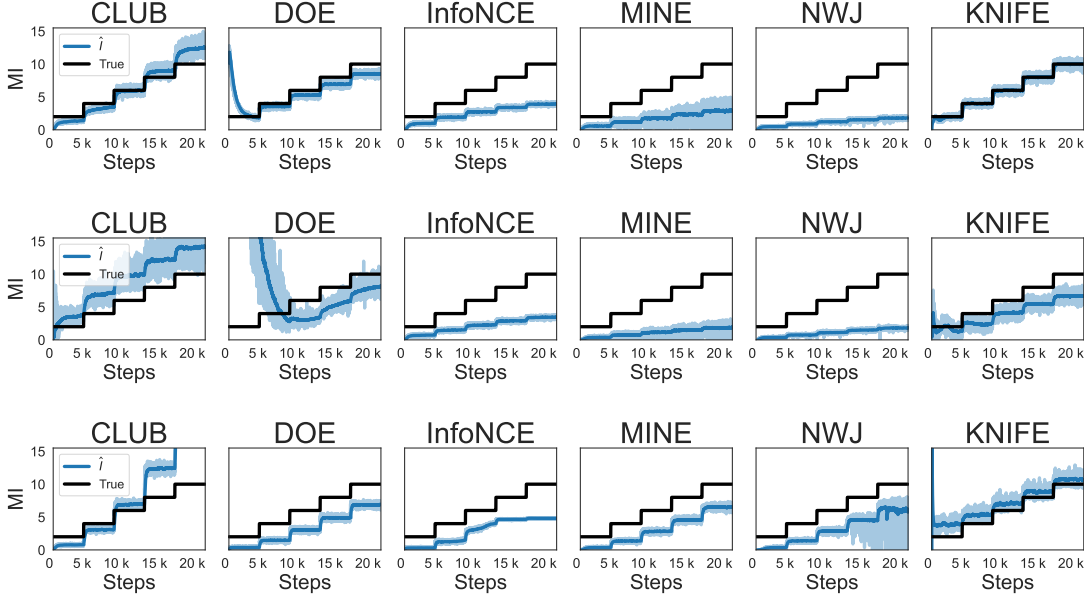

Figure 3: **Top:** Estimation of  $I(X^d; Y^d)$ , where  $(X, Y)$  are multivariate Gaussian with correlation coefficient  $\rho_i$  in the  $i$ -th epoch and  $d = 20$ . **Middle:** Estimation of  $I(X^d; (Y^3)^d)$ . **Bottom:** Estimation of  $I(X^d; Y^d)$  for uniform  $(X, E)$  and  $Y = \rho_i X + \sqrt{1 - \rho_i^2} E$  in the  $i$ -th epoch.

## 4 Experiments on Natural Data

In this section, we benchmark our proposed KNIFE-based MI estimator on three practical applications, spanning textual and visual data. We reproduce and compare our method to the most recent MI estimators including MINE [31], NWJ [32], and InfoNCE [16].

**Common notation:** In all following applications, we will use  $\Phi_\psi: \mathcal{X} \rightarrow \mathcal{Z}$  to denote an encoder, where  $\mathcal{X}$  is the raw input space (i.e., texts or images), and  $\mathcal{Z}$  denotes a lower dimensional continuous feature space. Additionally, we will use  $C_\psi: \mathcal{Z} \rightarrow \mathcal{Y}$  to denote a shallow classifier from the latent space  $\mathcal{Z}$  to a discrete or continuous target space  $\mathcal{Y}$  for classification or regression, respectively. We will use  $\psi$  to denote the parameters of both models,  $\Phi_\psi$  and  $C_\psi$ .

### 4.1 Information Bottleneck for Language Model Finetuning

The Information Bottleneck (IB) [52] has recently been applied to fine-tune large-scale pretrained models [27] such as BERT [28]. In this scenario, the IB method aims at suppressing irrelevant features in order to reduce overfitting. Formally, given textual input  $X \in \mathcal{X}$  and a target label  $Y \in \mathcal{Y}$ , the goal is to learn the encoder  $\Phi_\psi$  and classifier  $C_\psi$ , such that  $\Phi_\psi(X)$  retains little information about  $X$ , while still producing discriminative features, allowing the prediction of  $Y$ . Thus, the goal is to minimize the following loss function

$$\mathcal{L} = \lambda \cdot \underbrace{I(\Phi_\psi(X); X)}_{\text{compression term}} - \underbrace{I(\Phi_\psi(X); Y)}_{\text{downstream term}}, \quad (11)$$

where  $\lambda$  controls the trade-off between the downstream and the compression terms.

**Setup:** Following [27], we work with the VIBERT model (based on BERT), which uses a Gaussian distribution as prior.  $\Phi_\psi$  is implemented as a stochastic encoder  $\Phi_\psi(X) = Z \sim \mathcal{N}(\mu_\psi(X), \Sigma_\psi(X))$ . Details on the architecture of  $\mu_\psi$  and  $\Sigma_\psi$  can be found in the supplementary material. The classifier  $C_\psi$  is composed of dense layers. To minimize (11), the second part of the objective is bounded using the variational bound from [12]. Since we use a Gaussian prior,  $h(Z|X)$  can be expressed in closed form.<sup>2</sup> Thus, when using KNIFE,  $I(X; Z) = h(Z) - h(Z|X)$  can be estimated by using  $\hat{h}_{\text{KNIFE}}$

<sup>2</sup> $h(Z|X) = \frac{1}{2} \ln |\Sigma_\psi(X)| + \frac{d}{2} \ln(2\pi e)$ , where  $d$  is the dimension of  $X$  and  $|\cdot|$  denotes the determinant.

Table 1: Fine-tuning on GLUE. Following [58, 59], mean and variance are computed for 10 seeds.

|              | MRPC                  |                       | STS-B                 |                       | RTE                   |
|--------------|-----------------------|-----------------------|-----------------------|-----------------------|-----------------------|
|              | Accuracy              | F1                    | Pearson               | Spearman              | Accuracy              |
| BERT [28]    | 83.4 $\pm$ 0.9        | 88.2 $\pm$ 0.7        | 89.2 $\pm$ 0.4        | 88.8 $\pm$ 0.4        | 69.4 $\pm$ 0.4        |
| CLUB [30]    | 85.0 $\pm$ 0.4        | 89.0 $\pm$ 0.7        | 89.7 $\pm$ 0.2        | 89.4 $\pm$ 0.1        | 70.7 $\pm$ 0.1        |
| InfoNCE [16] | 84.9 $\pm$ 0.8        | 88.9 $\pm$ 0.6        | 89.4 $\pm$ 0.4        | 89.7 $\pm$ 0.6        | 70.6 $\pm$ 0.1        |
| MINE [31]    | 80.0 $\pm$ 2.5        | 85.0 $\pm$ 0.9        | 88.0 $\pm$ 0.7        | 88.0 $\pm$ 0.6        | 69.0 $\pm$ 0.9        |
| NWJ [32]     | 84.6 $\pm$ 0.8        | 88.1 $\pm$ 0.7        | 89.8 $\pm$ 0.1        | 89.6 $\pm$ 0.2        | 69.6 $\pm$ 0.7        |
| VUB [29]     | 85.1 $\pm$ 0.5        | 89.1 $\pm$ 0.3        | 90.0 $\pm$ 0.2        | 89.5 $\pm$ 0.3        | 70.9 $\pm$ 0.1        |
| KNIFE        | <b>85.3</b> $\pm$ 0.1 | <b>90.1</b> $\pm$ 0.1 | <b>90.3</b> $\pm$ 0.0 | <b>90.1</b> $\pm$ 0.0 | <b>72.3</b> $\pm$ 0.2 |

to estimate  $h(Z)$ . We compare this KNIFE-based MI estimator with different baselines: CLUB, InfoNCE, MINE, NWJ, and the variational upper bound (VUB). For completeness, we also compare all these models against a BERT model trained by minimization of a cross-entropy loss.

We closely follow the protocol of [27] and work on the GLUE benchmark [53] originally composed of 5 datasets. However, following [27], we choose to finetune neither on WNLI [54] nor on CoLA [55] due to reported flaws in these datasets.<sup>3</sup> The evaluation is carried out on the standard validation splits as the test splits are not available. Following standard practice [56, 57], we report the accuracy and the F1 for MRPC, the accuracy for RTE and the Pearson and Spearman correlation coefficient for STS-B.

**Results:** Table 1 reports our results on the GLUE benchmark. We observe that KNIFE obtains the best results on all three datasets and the lowest variance on MRPC and STS-B. The use of a Gaussian prior in the stochastic encoder  $\Phi_\psi$  could explain the observed improvement of KNIFE-based estimation over MI-estimators such as CLUB, InfoNCE, MINE, or NWJ.

## 4.2 Fair Textual Classification

In the fair classification task, we would like to take a decision without utilizing private information such as gender, age, or race. For this task, MI can be minimized to disentangle the output of the encoder  $Z$  and a private label  $S \in \mathcal{S}$  (e.g., gender, age, or race).

**Goal:** Given an input text  $X$ , a discrete target label  $Y$  and a private label  $S$ , the goal is to minimize the loss

$$\mathcal{L} = \underbrace{\text{CE}(Y; \Phi_\psi(X))}_{\text{downstream task}} + \lambda \cdot \underbrace{\text{I}(\Phi_\psi(X); S)}_{\text{disentangled}}, \quad (12)$$

where  $\lambda$  is a meta-parameter that controls the trade-off between minimizing MI and minimizing the Cross Entropy (CE) loss. In this framework, a classifier is said to be fair or to achieve perfect privacy if no statistical information about  $S$  can be extracted from  $\Phi_\psi(X)$ . Overall, a good model should achieve high accuracy on the main task (i.e., prediction of  $Y$ ) while removing information about the protected attribute  $S$ . This information is measured by training an offline classifier to recover the protected attribute  $S$ .

**Setup:** We compute the second term of (12) with competing MI estimators, as well as the model from [60], which will be referred to as “Adv”, as it boils down to training an adversary to recover the private label from the latent representation  $Z$ . For KNIFE-based MI estimation, we use two differential entropy estimators (as  $S$  is a binary label), following the approach outlined in Section 2.2. All derivations are detailed in the supplementary material.

We follow the experimental setting from [60, 61] and use two datasets from the DIAL corpus [62] (over 50 million tweets) where the protected attribute  $S$  is the race and the main labels are sentiment or mention labels. The mention label indicates whether a tweet is conversational or not. We follow the official split using 160 000 tweets for training and two additional sets composed of 10 000 tweets each for development and testing. In all cases, the labels  $S$  and  $Y$  are binary and balanced, thus a random guess corresponds to 50% accuracy.

<sup>3</sup>see <https://gluebenchmark.com/faq>

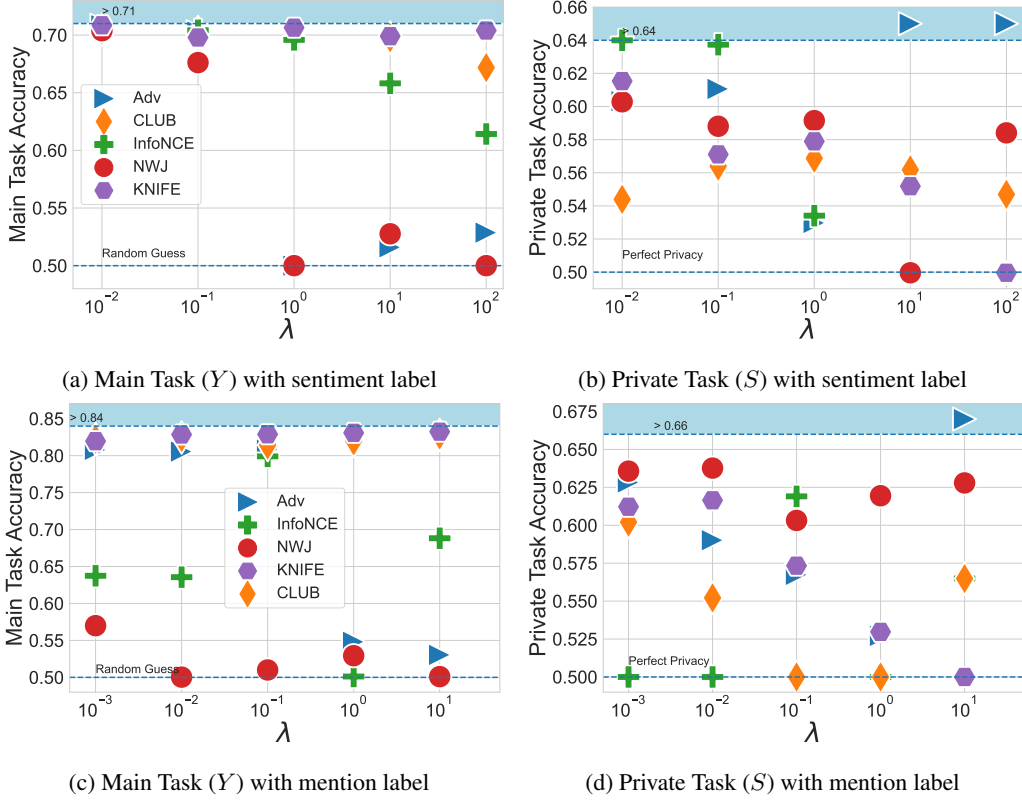

Figure 4: Results on the fair classification task for both main (Figures 4a and 4c) and private task (Figures 4b and 4d) for both mention and sentiment labels. Results of MINE are not reported because of instabilities that prevent the network from converging. Figures 4b and 4d are obtained by training an offline classifier to recover the protected attribute  $S$  from  $\Phi_\psi(X)$ .

**Results:** Figure 4 gathers results on the fair classification task. The upper dashed lines represent the (private and main) task accuracies when training a model with only the CE loss (case  $\lambda = 0$  in (12)). This shows that the learned encoding  $\Phi_\psi(X)$  contains information about the protected attribute, when training is only performed for the main task. On both the sentiment and mention task, we observe that a KNIFE-based estimator can achieve perfect privacy (see Figures 4b and 4d) with nearly no accuracy loss in the main task (see Figures 4a and 4c). For other MI estimators, we observe a different behavior on the two tasks. For sentiment labels, most MI estimators fail to reach perfect privacy (e.g., CLUB, NWJ, and Adv) while others (e.g., InfoNCE) achieve perfect privacy while degrading the main task accuracy (10% loss on main accuracy). For mention labels, CLUB can also reach perfect privacy with almost no degradation of the accuracy of the main task. Overall, it is worth noting that KNIFE-based MI estimators enable a better control of the degree of disentanglement than the reported baselines.

### 4.3 Unsupervised Domain Adaptation

In unsupervised domain adaptation, the goal is to transfer knowledge from the source domain ( $S$ ) with a potentially large number of labeled examples to a target domain ( $T$ ), where only unlabeled examples are available.

**Goal:** Specifically, the learner is given access to labeled images from a source domain  $(x_s, y) \sim (X_S, Y) \in \mathcal{X}_S \times \mathcal{Y}$  and unlabeled images from a target domain  $x_t \sim X_T \in \mathcal{X}_T$ . The goal is to learn a classification model  $\{\Phi_\psi, C_\psi\}$  that generalizes well to the target domain. Training models on the supervised source data only results in domain-specific latent representations  $\Phi_\psi(X)$  leading to poor generalization ( $X$  is chosen randomly from  $\{X_S, X_T\}$ ). In order to make the latent representations as domain-agnostic as possible, we follow the information-theoretic method proposed by [63], and

Table 2: Domain adaptation results: M (MNIST), MM (MNIST M), U (USPS), SV (SVHN), C (CIFAR10) and S (STL10). Results are averaged over 3 seeds.

|             | M $\rightarrow$ MM    | S $\rightarrow$ C     | U $\rightarrow$ M     | M $\rightarrow$ U     | C $\rightarrow$ S     | SV $\rightarrow$ M    | Mean                  |
|-------------|-----------------------|-----------------------|-----------------------|-----------------------|-----------------------|-----------------------|-----------------------|
| Source only | 51.9 $\pm$ 0.8        | 58.3 $\pm$ 0.2        | 91.1 $\pm$ 0.7        | 93.5 $\pm$ 0.6        | <b>72.3</b> $\pm$ 0.5 | 54.7 $\pm$ 2.8        | 70.3 $\pm$ 0.9        |
| CLUB        | <b>79.1</b> $\pm$ 2.2 | 59.9 $\pm$ 1.9        | 96.0 $\pm$ 0.2        | 96.8 $\pm$ 0.5        | 71.6 $\pm$ 1.3        | 83.8 $\pm$ 3.4        | 81.2 $\pm$ 1.7        |
| INFONCE     | 77.3 $\pm$ 0.5        | 61.0 $\pm$ 0.1        | 97.4 $\pm$ 0.2        | 97.0 $\pm$ 0.3        | 70.6 $\pm$ 0.8        | 89.2 $\pm$ 4.1        | 82.1 $\pm$ 1.0        |
| MINE        | 76.7 $\pm$ 0.4        | 61.2 $\pm$ 0.3        | <b>97.7</b> $\pm$ 0.1 | 97.3 $\pm$ 0.1        | 70.8 $\pm$ 1.0        | 91.8 $\pm$ 0.8        | 82.6 $\pm$ 0.4        |
| NWJ         | 77.1 $\pm$ 0.6        | 61.2 $\pm$ 0.3        | 97.6 $\pm$ 0.1        | 97.3 $\pm$ 0.5        | 72.1 $\pm$ 0.7        | 91.4 $\pm$ 0.8        | 82.8 $\pm$ 0.5        |
| KNIFE       | 78.7 $\pm$ 0.7        | <b>61.8</b> $\pm$ 0.5 | <b>97.7</b> $\pm$ 0.3 | <b>97.4</b> $\pm$ 0.4 | 71.2 $\pm$ 1.8        | <b>93.2</b> $\pm$ 0.2 | <b>83.4</b> $\pm$ 0.6 |

used in [30]. The idea is to learn an additional binary model  $\{\Phi_\nu^d, C_\nu^d\}$ , whose goal is to guess the domain  $D \in \{0, 1\}$  of  $X$ . The latent representation learned by  $\Phi_\nu^d$  will therefore contain all the domain-specific information that we would like the main encoder  $\Phi_\psi$  to discard. In other words, we would like  $\Phi_\psi(X)$  and  $\Phi_\nu^d(X)$  to be completely disentangled, which naturally corresponds to a minimization of  $I(\Phi_\psi(X); \Phi_\nu^d(X))$ , the MI between those two representations. Concretely, the domain classifier is trained to minimize the CE between domain labels  $D$  and its own predictions, whereas the main classifier is trained to properly classify support samples while minimizing the MI between  $\Phi_\psi(X)$  and  $\Phi_\nu^d(X)$ . Using  $f_\nu^d := C_\nu^d \circ \Phi_\nu^d$  and  $f_\psi := C_\psi \circ \Phi_\psi$ , the objectives read

$$\min_{\nu} \text{CE}(D; f_\nu^d(X)) \quad \text{and} \quad \min_{\psi} \text{CE}(Y; f_\psi(X_S)) + \lambda \cdot I(\Phi_\psi(X); \Phi_\nu^d(X)). \quad (13)$$

**Setup:** The different MI estimators are compared based on their ability to guide training by estimating  $I(\Phi_\psi(X); \Phi_\nu^d(X))$  in (13). Following [30], we consider a total of 6 source/target scenarios formed with MNIST [64], MNIST-M [65], SVHN [66], CIFAR-10 [67], and STL-10 [68] datasets. We reproduce all methods in our framework, following the setup of [30] as closely as possible. The exhaustive list of fixed and tuned hyper-parameters can be found in the supplementary material.

**Results:** Results are presented in Table 2. The KNIFE-based estimator is able to outperform most recent tailored MI estimators in these challenging scenarios where both random variables  $\Phi_\psi(X)$  and  $\Phi_\nu^d(X)$  are continuous.

## 5 Concluding Remarks and Outlook

In this work, we introduced KNIFE a differentiable kernel-based estimator of differential entropy. KNIFE relies on a fully learnable kernel (i.e., weights, shifts, and covariance matrices) density estimator learned by SGD optimization. This allows for a flexible and efficient adaptation to the shape and multiple modes of the data distribution. KNIFE does not require distributional assumptions (other than smoothness) and can be used to construct estimators for conditional differential entropy and mutual information, where one random variable may be discrete.

Extensive experiments on synthetic data validate that KNIFE-based estimators outperform existing differential entropy and MI estimators. On real dataset, for representation learning tasks such as pretrained language model finetuning, fair textual classification, and visual domain adaptation, our experiments demonstrate the superior performance of KNIFE. Even though our experiments focused on MI estimation, primarily to facilitate comparison with the existing literature, we believe that KNIFE can pave the way towards new applications of differential entropy estimation in its own right.

Despite the fundamental challenges in the problem of differential entropy estimation, beyond limitations arising from the use of a finite number of samples, KNIFE has demonstrated promising empirical results in various representation learning tasks. Interestingly, KNIFE exhibits an inherent ability to rapidly adapt to changes in the underlying data distribution. In future work, we hope to formally derive statistical guarantees for KNIFE under mild smoothness conditions on the underlying data distribution by bounding the error as a function of the increasing sample size and the kernel-class.

## References

- [1] C. E. Shannon, “A mathematical theory of communication,” *The Bell System Technical Journal*, vol. 27, no. 3, pp. 379–423, Jul. 1948.
- [2] R. Linsker, “How to generate ordered maps by maximizing the mutual information between input and output signals,” in *Neural Comput.*, 1989.
- [3] K. Torkkola, *Information-Theoretic Methods*. Berlin, Heidelberg: Springer Berlin Heidelberg, 2006, pp. 167–185. [Online]. Available: [https://doi.org/10.1007/978-3-540-35488-8\\_7](https://doi.org/10.1007/978-3-540-35488-8_7)
- [4] P. Shyam, W. Jaśkowski, and F. Gomez, “Model-based active exploration,” in *Proceedings of the 36th International Conference on Machine Learning*, ser. Proceedings of Machine Learning Research, K. Chaudhuri and R. Salakhutdinov, Eds., vol. 97. PMLR, 09–15 Jun 2019, pp. 5779–5788. [Online]. Available: <http://proceedings.mlr.press/v97/shyam19a.html>
- [5] E. Hazan, S. Kakade, K. Singh, and A. Van Soest, “Provably efficient maximum entropy exploration,” vol. 97, pp. 2681–2691, 09–15 Jun 2019. [Online]. Available: <http://proceedings.mlr.press/v97/hazan19a.html>
- [6] Z. Ahmed, N. Le Roux, M. Norouzi, and D. Schuurmans, “Understanding the impact of entropy on policy optimization,” vol. 97, pp. 151–160, 09–15 Jun 2019. [Online]. Available: <http://proceedings.mlr.press/v97/ahmed19a.html>
- [7] H. Kim, J. Kim, Y. Jeong, S. Levine, and H. O. Song, “EMI: exploration with mutual information,” vol. 97, pp. 3360–3369, 2019. [Online]. Available: <http://proceedings.mlr.press/v97/kim19a.html>
- [8] A. Kraskov, H. Stögbauer, and P. Grassberger, “Estimating mutual information,” *Phys. Rev. E*, vol. 69, p. 066138, Jun 2004. [Online]. Available: <https://link.aps.org/doi/10.1103/PhysRevE.69.066138>
- [9] G. Pichler, P. Piantanida, and G. Koliander, “On the estimation of information measures of continuous distributions,” *CoRR*, vol. abs/2002.02851, 2020. [Online]. Available: <https://arxiv.org/abs/2002.02851>
- [10] D. McAllester and K. Stratos, “Formal limitations on the measurement of mutual information,” in *Proceedings of the Twenty Third International Conference on Artificial Intelligence and Statistics*, ser. Proceedings of Machine Learning Research, S. Chiappa and R. Calandra, Eds., vol. 108. PMLR, 26–28 Aug 2020, pp. 875–884. [Online]. Available: <http://proceedings.mlr.press/v108/mcallester20a.html>
- [11] B. Poole, S. Ozair, A. Van Den Oord, A. Alemi, and G. Tucker, “On variational bounds of mutual information,” in *Proceedings of the 36th International Conference on Machine Learning*, ser. Proceedings of Machine Learning Research, K. Chaudhuri and R. Salakhutdinov, Eds., vol. 97. PMLR, 09–15 Jun 2019, pp. 5171–5180. [Online]. Available: <http://proceedings.mlr.press/v97/poole19a.html>
- [12] D. Barber and F. Agakov, “The im algorithm: A variational approach to information maximization,” in *Proceedings of the 16th International Conference on Neural Information Processing Systems*, ser. NIPS’03. Cambridge, MA, USA: MIT Press, 2003, p. 201–208.
- [13] R. Linsker, “Self-organization in a perceptual network,” in *Computer*, 1988.
- [14] A. Krause, P. Perona, and R. Gomes, “Discriminative clustering by regularized information maximization,” in *Advances in Neural Information Processing Systems*, J. Lafferty, C. Williams, J. Shawe-Taylor, R. Zemel, and A. Culotta, Eds., vol. 23. Curran Associates, Inc., 2010. [Online]. Available: <https://proceedings.neurips.cc/paper/2010/file/42998cf32d552343bc8e460416382dca-Paper.pdf>
- [15] J. Bridle, A. Heading, and D. MacKay, “Unsupervised classifiers, mutual information and ‘phantom targets,’” in *Advances in Neural Information Processing Systems*, J. Moody, S. Hanson, and R. P. Lippmann, Eds., vol. 4. Morgan-Kaufmann, 1992. [Online]. Available: <https://proceedings.neurips.cc/paper/1991/file/a8abb4bb284b5b27aa7cb790dc20f80b-Paper.pdf>
- [16] A. van den Oord, Y. Li, and O. Vinyals, “Representation learning with contrastive predictive coding,” *CoRR*, vol. abs/1807.03748, 2018. [Online]. Available: <http://arxiv.org/abs/1807.03748>
- [17] R. D. Hjelm, A. Fedorov, S. Lavoie-Marchildon, K. Grewal, P. Bachman, A. Trischler, and Y. Bengio, “Learning deep representations by mutual information estimation and maximization,” 2019. [Online]. Available: <https://openreview.net/forum?id=Bklr3j0cKX>

- [18] R. T. Q. Chen, X. Li, R. B. Grosse, and D. K. Duvenaud, “Isolating sources of disentanglement in variational autoencoders,” vol. 31, 2018. [Online]. Available: <https://proceedings.neurips.cc/paper/2018/file/1ee3dfcd8a0645a25a35977997223d22-Paper.pdf>
- [19] A. Anand, E. Racah, S. Ozair, Y. Bengio, M.-A. Côté, and R. D. Hjelm, “Unsupervised state representation learning in atari,” in *Advances in Neural Information Processing Systems*, H. Wallach, H. Larochelle, A. Beygelzimer, F. d’Alché-Buc, E. Fox, and R. Garnett, Eds., vol. 32. Curran Associates, Inc., 2019. [Online]. Available: <https://proceedings.neurips.cc/paper/2019/file/6fb52e71b837628ac16539c1ff911667-Paper.pdf>
- [20] M. Tschannen, J. Djolonga, P. K. Rubenstein, S. Gelly, and M. Lucic, “On mutual information maximization for representation learning,” in *International Conference on Learning Representations*, 2020. [Online]. Available: <https://openreview.net/forum?id=rkxoh24FPH>
- [21] W. Hu, T. Miyato, S. Tokui, E. Matsumoto, and M. Sugiyama, “Learning discrete representations via information maximizing self-augmented training,” in *Proceedings of the 34th International Conference on Machine Learning*, ser. Proceedings of Machine Learning Research, D. Precup and Y. W. Teh, Eds., vol. 70. PMLR, 06–11 Aug 2017, pp. 1558–1567. [Online]. Available: <http://proceedings.mlr.press/v70/hu17b.html>
- [22] X. Ji, J. F. Henriques, and A. Vedaldi, “Invariant information clustering for unsupervised image classification and segmentation,” in *Proceedings of the IEEE/CVF International Conference on Computer Vision (ICCV)*, October 2019.
- [23] X. Chen, Y. Duan, R. Houthoofd, J. Schulman, I. Sutskever, and P. Abbeel, “Infogan: Interpretable representation learning by information maximizing generative adversarial nets,” p. 2180–2188, 2016.
- [24] S. Zhao, J. Song, and S. Ermon, “Infovae: Information maximizing variational autoencoders,” *ArXiv*, vol. abs/1706.02262, 2017.
- [25] P. Cheng, M. R. Min, D. Shen, C. Malon, Y. Zhang, Y. Li, and L. Carin, “Improving disentangled text representation learning with information-theoretic guidance,” *arXiv preprint arXiv:2006.00693*, 2020.
- [26] P. Colombo, C. Clavel, and P. Piantanida, “A novel estimator of mutual information for learning to disentangle textual representations,” *arXiv preprint arXiv:2105.02685*, 2021.
- [27] R. K. Mahabadi, Y. Belinkov, and J. Henderson, “Variational information bottleneck for effective low-resource fine-tuning,” *ICLR. OpenReview. net*, 2021.
- [28] J. Devlin, M.-W. Chang, K. Lee, and K. Toutanova, “Bert: Pre-training of deep bidirectional transformers for language understanding,” *arXiv preprint arXiv:1810.04805*, 2018.
- [29] A. A. Alemi, I. Fischer, J. V. Dillon, and K. Murphy, “Deep variational information bottleneck,” *CoRR*, vol. abs/1612.00410, 2016. [Online]. Available: <http://arxiv.org/abs/1612.00410>
- [30] P. Cheng, W. Hao, S. Dai, J. Liu, Z. Gan, and L. Carin, “CLUB: A contrastive log-ratio upper bound of mutual information,” vol. 119, pp. 1779–1788, 13–18 Jul 2020. [Online]. Available: <http://proceedings.mlr.press/v119/cheng20b.html>
- [31] I. Belghazi, S. Rajeswar, A. Baratin, R. D. Hjelm, and A. C. Courville, “MINE: mutual information neural estimation,” *CoRR*, vol. abs/1801.04062, 2018. [Online]. Available: <http://arxiv.org/abs/1801.04062>
- [32] X. Nguyen, M. J. Wainwright, and M. I. Jordan, “Estimating divergence functionals and the likelihood ratio by convex risk minimization,” *IEEE Transactions on Information Theory*, vol. 56, no. 11, pp. 5847–5861, 2010.
- [33] J. Beirlant, E. J. Dudewicz, L. Györfi, and E. C. Van der Meulen, “Nonparametric entropy estimation: An overview,” *International Journal of Mathematical and Statistical Sciences*, vol. 6, no. 1, pp. 17–39, 1997.
- [34] K. Hlaváčková-Schindler, M. Paluš, M. Vejmelka, and J. Bhattacharya, “Causality detection based on information-theoretic approaches in time series analysis,” *Physics Reports*, vol. 441, no. 1, pp. 1–46, 2007.
- [35] S. Verdú, “Empirical estimation of information measures: A literature guide,” *Entropy*, vol. 21, no. 8, 2019. [Online]. Available: <https://www.mdpi.com/1099-4300/21/8/720>

- [36] I. Ahmad and P.-E. Lin, “A nonparametric estimation of the entropy for absolutely continuous distributions,” *IEEE Trans. Inf. Theory*, vol. 22, no. 3, pp. 372–375, May 1976.
- [37] L. Györfi and E. C. Van der Meulen, “Density-free convergence properties of various estimators of entropy,” *Computational Statistics & Data Analysis*, vol. 5, no. 4, pp. 425–436, 1987.
- [38] F. Tarasenko, “On the evaluation of an unknown probability density function, the direct estimation of the entropy from independent observations of a continuous random variable, and the distribution-free entropy test of goodness-of-fit,” *Proceedings of the IEEE*, vol. 56, no. 11, pp. 2052–2053, 1968.
- [39] L. Kozachenko and N. N. Leonenko, “Sample estimate of the entropy of a random vector,” *Problemy Peredachi Informatsii*, vol. 23, no. 2, pp. 9–16, 1987.
- [40] A. B. Tsybakov and E. C. Van der Meulen, “Root-n consistent estimators of entropy for densities with unbounded support,” *Scandinavian Journal of Statistics*, pp. 75–83, 1996.
- [41] Q. Wang, S. R. Kulkarni, and S. Verdú, “Universal estimation of information measures for analog sources,” *Foundations and Trends in Communications and Information Theory*, vol. 5, no. 3, pp. 265–353, 2009.
- [42] M. Rosenblatt, “Remarks on some nonparametric estimates of a density function,” *Ann. Math. Statist.*, vol. 27, no. 3, pp. 832–837, 1956.
- [43] E. Parzen, “On estimation of a probability density function and mode,” *The annals of mathematical statistics*, vol. 33, no. 3, pp. 1065–1076, 1962.
- [44] H. Joe, “Estimation of entropy and other functionals of a multivariate density,” *Annals of the Institute of Statistical Mathematics*, vol. 41, no. 4, pp. 683–697, 1989.
- [45] P. Hall and S. Morton, “On the estimation of entropy,” *Annals of the Institute of Statistical Mathematics*, vol. 45, pp. 69–88, Feb. 1993.
- [46] P. Viola, N. N. Schraudolph, and T. J. Sejnowski, “Empirical entropy manipulation for real-world problems,” *Advances in neural information processing systems*, pp. 851–857, 1996.
- [47] N. N. Schraudolph, “Gradient-based manipulation of nonparametric entropy estimates,” *IEEE Transactions on Neural Networks*, vol. 15, no. 4, pp. 828–837, 2004.
- [48] A. Kolchinsky and B. D. Tracey, “Estimating mixture entropy with pairwise distances,” *Entropy*, vol. 19, no. 7, p. 361, 2017.
- [49] Y. P. Chaubey and N. L. Vu, “On the estimation of entropy for non-negative data,” *Journal of Statistical Theory and Practice*, vol. 15, no. 2, pp. 1–19, 2021.
- [50] D. P. Kingma and J. Ba, “Adam: A method for stochastic optimization.”
- [51] I. Loshchilov and F. Hutter, “Decoupled weight decay regularization,” *arXiv preprint arXiv:1711.05101*, 2017.
- [52] N. Tishby, F. C. Pereira, and W. Bialek, “The information bottleneck method,” *arXiv preprint physics/0004057*, 2000.
- [53] A. Wang, A. Singh, J. Michael, F. Hill, O. Levy, and S. R. Bowman, “Glue: A multi-task benchmark and analysis platform for natural language understanding,” *arXiv preprint arXiv:1804.07461*, 2018.
- [54] L. Morgenstern and C. Ortiz, “The winograd schema challenge: Evaluating progress in commonsense reasoning,” in *Twenty-Seventh IAAI Conference*, 2015.
- [55] A. Warstadt, A. Singh, and S. R. Bowman, “Neural network acceptability judgments,” *Transactions of the Association for Computational Linguistics*, vol. 7, pp. 625–641, 2019.
- [56] Y. Liu, M. Ott, N. Goyal, J. Du, M. Joshi, D. Chen, O. Levy, M. Lewis, L. Zettlemoyer, and V. Stoyanov, “Roberta: A robustly optimized bert pretraining approach,” *arXiv preprint arXiv:1907.11692*, 2019.
- [57] Z. Yang, Z. Dai, Y. Yang, J. Carbonell, R. Salakhutdinov, and Q. V. Le, “Xlnet: Generalized autoregressive pretraining for language understanding,” *arXiv preprint arXiv:1906.08237*, 2019.
- [58] C. Lee, K. Cho, and W. Kang, “Mixout: Effective regularization to finetune large-scale pretrained language models,” *arXiv preprint arXiv:1909.11299*, 2019.

- 460 [59] J. Dodge, G. Ilharco, R. Schwartz, A. Farhadi, H. Hajishirzi, and N. Smith, “Fine-tuning  
461 pretrained language models: Weight initializations, data orders, and early stopping,” *arXiv*  
462 *preprint arXiv:2002.06305*, 2020.
- 463 [60] Y. Elazar and Y. Goldberg, “Adversarial removal of demographic attributes from text data,”  
464 *arXiv preprint arXiv:1808.06640*, 2018.
- 465 [61] M. Barrett, Y. Kementchedjieva, Y. Elazar, D. Elliott, and A. Søgaard, “Adversarial removal  
466 of demographic attributes revisited,” in *Proceedings of the 2019 Conference on Empirical*  
467 *Methods in Natural Language Processing and the 9th International Joint Conference on Natural*  
468 *Language Processing (EMNLP-IJCNLP)*, 2019, pp. 6331–6336.
- 469 [62] S. L. Blodgett, L. Green, and B. O’Connor, “Demographic dialectal variation in social media:  
470 A case study of african-american english,” *arXiv preprint arXiv:1608.08868*, 2016.
- 471 [63] B. Gholami, P. Sahu, O. Rudovic, K. Bousmalis, and V. Pavlovic, “Unsupervised multi-target do-  
472 main adaptation: An information theoretic approach,” *IEEE Transactions on Image Processing*,  
473 vol. 29, pp. 3993–4002, 2020.
- 474 [64] Y. LeCun and C. Cortes, “MNIST handwritten digit database,” 2010. [Online]. Available:  
475 <http://yann.lecun.com/exdb/mnist/>
- 476 [65] Y. Ganin, E. Ustinova, H. Ajakan, P. Germain, H. Larochelle, F. Laviolette, M. Marchand,  
477 and V. Lempitsky, “Domain-adversarial training of neural networks,” *The journal of machine*  
478 *learning research*, vol. 17, no. 1, pp. 2096–2030, 2016.
- 479 [66] Y. Netzer, T. Wang, A. Coates, A. Bissacco, B. Wu, and A. Y. Ng, “Reading digits in natural  
480 images with unsupervised feature learning,” 2011.
- 481 [67] A. Krizhevsky, G. Hinton *et al.*, “Learning multiple layers of features from tiny images,” 2009.
- 482 [68] A. Coates, A. Ng, and H. Lee, “An analysis of single-layer networks in unsupervised feature  
483 learning,” in *Proceedings of the fourteenth international conference on artificial intelligence*  
484 *and statistics. JMLR Workshop and Conference Proceedings*, 2011, pp. 215–223.

## Checklist

### 1. For all authors...

- (a) Do the main claims made in the abstract and introduction accurately reflect the paper's contributions and scope? [Yes]
- (b) Did you describe the limitations of your work? [Yes]
- (c) Did you discuss any potential negative societal impacts of your work? [N/A]
- (d) Have you read the ethics review guidelines and ensured that your paper conforms to them? [Yes]

### 2. If you are including theoretical results...

- (a) Did you state the full set of assumptions of all theoretical results? [N/A]
- (b) Did you include complete proofs of all theoretical results? [N/A]

### 3. If you ran experiments...

- (a) Did you include the code, data, and instructions needed to reproduce the main experimental results (either in the supplemental material or as a URL)? [Yes] in the supplementary material.
- (b) Did you specify all the training details (e.g., data splits, hyperparameters, how they were chosen)? [Yes] in the supplementary material
- (c) Did you report error bars (e.g., with respect to the random seed after running experiments multiple times)? [Yes] We report the standard deviation in the result tables. Bias, variance and MSE are reported in the supplementary material.
- (d) Did you include the total amount of compute and the type of resources used (e.g., type of GPUs, internal cluster, or cloud provider)? [Yes] in the supplementary material

### 4. If you are using existing assets (e.g., code, data, models) or curating/releasing new assets...

- (a) If your work uses existing assets, did you cite the creators? [Yes]
- (b) Did you mention the license of the assets? [Yes] It is provided in the README file of the supplementary code.
- (c) Did you include any new assets either in the supplemental material or as a URL? [Yes] Code is included in the supplementary material.
- (d) Did you discuss whether and how consent was obtained from people whose data you're using/curating? [N/A]
- (e) Did you discuss whether the data you are using/curating contains personally identifiable information or offensive content? [N/A]

### 5. If you used crowdsourcing or conducted research with human subjects...

- (a) Did you include the full text of instructions given to participants and screenshots, if applicable? [N/A]
- (b) Did you describe any potential participant risks, with links to Institutional Review Board (IRB) approvals, if applicable? [N/A]
- (c) Did you include the estimated hourly wage paid to participants and the total amount spent on participant compensation? [N/A]

## A Experimental Details of Experiments with Synthetic Data

### A.1 Differential Entropy Estimation of Gaussian Data

In Section 3.1.1, the estimation of the entropy  $h(X) = \frac{d}{2} \log 2\pi e$  for  $X \sim \mathcal{N}(\mathbf{0}, I_d)$  was performed with the hyperparameters given in Table 3. The mean error and its empirical standard deviation are reported over 20 runs, where an independently drawn evaluation set is used that has the same size as the training set.

In the experiment depicted in Figure 1, entropy is decreased after every epoch by letting  $X_i \sim \mathcal{N}(\mathbf{0}, a^i I_d)$ , where  $i = 0, \dots, 4$  is the epoch index. That is,  $X_i = \sqrt{a^i} G^d$ , where  $G$  is a standard normal random variable, resulting in an decrease of the differential entropy by  $\Delta = -\frac{d}{2} \log a \approx 22.18$  for  $a = \frac{1}{2}$  with every epoch. We start at  $h(X_0) = \frac{d}{2} \log 2\pi e \approx 90.81$  and successively decrease until  $h(X_4) = h(X_0) + 4\Delta \approx 2.1$ . Additional parameters can be found in Table 4.

**Computational Resources.** Training was performed on an NVidia V100 GPU. Taken together, training for the first experiments of entropy estimation in dimensions  $d = 10, 64$ , as well as the experiment depicted in Figure 1 used GPU time of less than 5 minutes.

### A.2 Differential Entropy Estimation of Triangle Mixtures

In Section 3.1.2, we perform an estimation of the entropy of  $c$ -component triangle mixture distributions. The pdf of such a  $c$ -component triangle-mixture, is given by

$$p(x) = \sum_{i=1}^c w_i \Lambda_{s_i} \left( x - i - \frac{1}{2} \right), \quad (14)$$

where  $\Lambda_s(x) := \frac{1}{s} \max\{0, 2 - 4s|x|\}$  is a centered triangle pdf with width  $s > 0$ . The scales  $\mathbf{s} = (s_1, \dots, s_c)$  and weights  $\mathbf{w} = (w_1, \dots, w_c)$  satisfy  $0 < s_i, w_i < 1$  and  $\sum_{i=1}^c w_i = 1$ . Before the experiment, we choose  $\mathbf{w}$  uniformly at random from the  $c$ -probability simplex and the scales are chosen uniformly at random in  $[0.1, 1.0]$ . An example for  $c = 10$  is the true pdf depicted in Figure 2 (left). For  $d > 1$ , we perform the estimation on  $d$  i.i.d. copies. Note that the triangle mixture with  $c$  components in  $d$ -dimensional space has  $c^d$  modes, i.e., the support can be partitioned into  $c^d$  disjoint components.

The parameters of the experiment yielding Figure 2 (left) are given in Table 5, while the details of the experiment depicted in Figure 2 (right) can be found in Table 6. The reported accuracy and standard deviation is empirically calculated over all 10 runs, where the evaluation set is independent of the training set and has the same size as the training set.

Table 3: Experimental details of first experiment in Section 3.1.1.

| Parameter               | Value                                 |
|-------------------------|---------------------------------------|
| Source Distribution $X$ | $X \sim \mathcal{N}(\mathbf{0}, I_d)$ |
| Dimension $d$           | 10 and 64                             |
| Optimizer               | Adam [50]                             |
| Learning Rate           | 0.01                                  |
| Batch Size $N$          | 128                                   |
| Kernel Size $M$         | 128                                   |
| Iterations per epoch    | 200                                   |
| Epochs                  | 1                                     |
| Runs                    | 20                                    |

Table 4: Experimental details of the experiment depicted in Figure 1.

| Parameter               | Value                                                              |
|-------------------------|--------------------------------------------------------------------|
| Source Distribution $X$ | $X \sim \mathcal{N}(\mathbf{0}, a^i I_d)$<br>for $i = 0, \dots, 4$ |
| Dimension $d$           | 64                                                                 |
| Factor $a$              | $\frac{1}{2}$                                                      |
| Optimizer               | Adam [50]                                                          |
| Learning Rate           | 0.01                                                               |
| Batch Size $N$          | 128                                                                |
| Kernel Size $M$         | 128                                                                |
| Iterations per epoch    | 1000                                                               |
| Epochs                  | 5                                                                  |
| Runs                    | 1                                                                  |

Table 5: Experimental details of the experiment resulting in the pdf in Figure 2 (left).

| Parameter               | Value                            |
|-------------------------|----------------------------------|
| Source Distribution $X$ | $c$ -component triangle mixtures |
| Components $c$          | 10                               |
| Dimension $d$           | 1                                |
| Optimizer               | Adam [50]                        |
| Learning Rate           | 0.1                              |
| Batch Size $N$          | 128                              |
| Kernel Size $M$         | 128                              |
| Iterations per epoch    | 100                              |
| Epochs                  | 10                               |
| Runs                    | 1                                |

Table 6: Experimental details of the experiment resulting in the training depicted in Figure 2 (right).

| Parameter               | Value                            |
|-------------------------|----------------------------------|
| Source Distribution $X$ | $c$ -component triangle mixtures |
| Components $c$          | 2                                |
| Dimension $d$           | 8                                |
| Optimizer               | Adam [50]                        |
| Learning Rate           | 0.001                            |
| Batch Size $N$          | 128                              |
| Kernel Size $M$         | 128                              |
| Iterations per epoch    | 1000                             |
| Epochs                  | 20                               |
| Runs                    | 10                               |

Table 7: Experimental details of the training depicted in Figure 3 (bottom).

| Parameter            | Value                      |
|----------------------|----------------------------|
| Dimension $d$        | 20                         |
| Optimizer            | Adam [50]                  |
| Learning Rates       | 0.01, 0.003, 0.001, 0.0003 |
| Batch Size $N$       | 128                        |
| Kernel Size $M$      | 128                        |
| Iterations per epoch | 20 000                     |
| Epochs               | 1                          |
| Runs                 | 10                         |

**Computational Resources.** Training was performed on an NVidia V100 GPU. Training in  $d = 1$  dimension, that resulted in Figure 2 (left) can be performed in seconds, while all training required for producing Figure 2 (right) used approximately 1.5 hours of GPU time.

### A.3 Mutual Information Estimation

In Section 3.1.1, we estimate  $I(X^d; Y^d)$  and  $I(X^d; (Y^3)^d)$  where  $(X, Y)$  are multivariate correlated Gaussian distributions. All neural networks are randomly initialized. The bias, variance, and MSE during training, as a function of the MI, can be observed in Figure 5.

In Section 3.2.2, we estimate  $I(X^d; Y^d)$  where  $X, E \sim \mathcal{U}[-\sqrt{3}, \sqrt{3}]$  are independent and  $Y$  is given by  $Y = \rho X + \sqrt{1 - \rho^2} E$  with  $0 < \rho < 1$ . The estimation is performed in 10 runs, randomly choosing the training meta-parameters as proposed by [10]. In Figure 3 (bottom), we present the best run for each method, selected by distance from the true MI at the end of training. The bias, variance, and MSE during training, as a function of the MI, can be observed in Figure 6. Details about the source distribution as well as details of the experiments can be found in Table 7. During experimentation it turned out to be beneficial to train the parameters  $\Theta$  and  $\theta$  in (10) separately and substantially increase the learning rate for the training of  $\theta$ . Thus, we increase the learning rate for the training of  $\theta$  by a factor of  $10^3$ .

**Model Architecture for  $\Theta$ .** We utilize the feed-forward architecture, also used in [10]. It is a simple architecture with two linear layers, one hidden layer using tanh activation, immediately followed by an output layer. The number of neurons in the hidden layer is a meta-parameter selected randomly from  $\{64, 128, 256\}$  for each training run. Three models with this architecture are used for the three parameters  $(\mathbf{A}, \mathbf{a}, \mathbf{u})$ , as described by (6), where only the output dimension is changed to fit the parameter dimension.

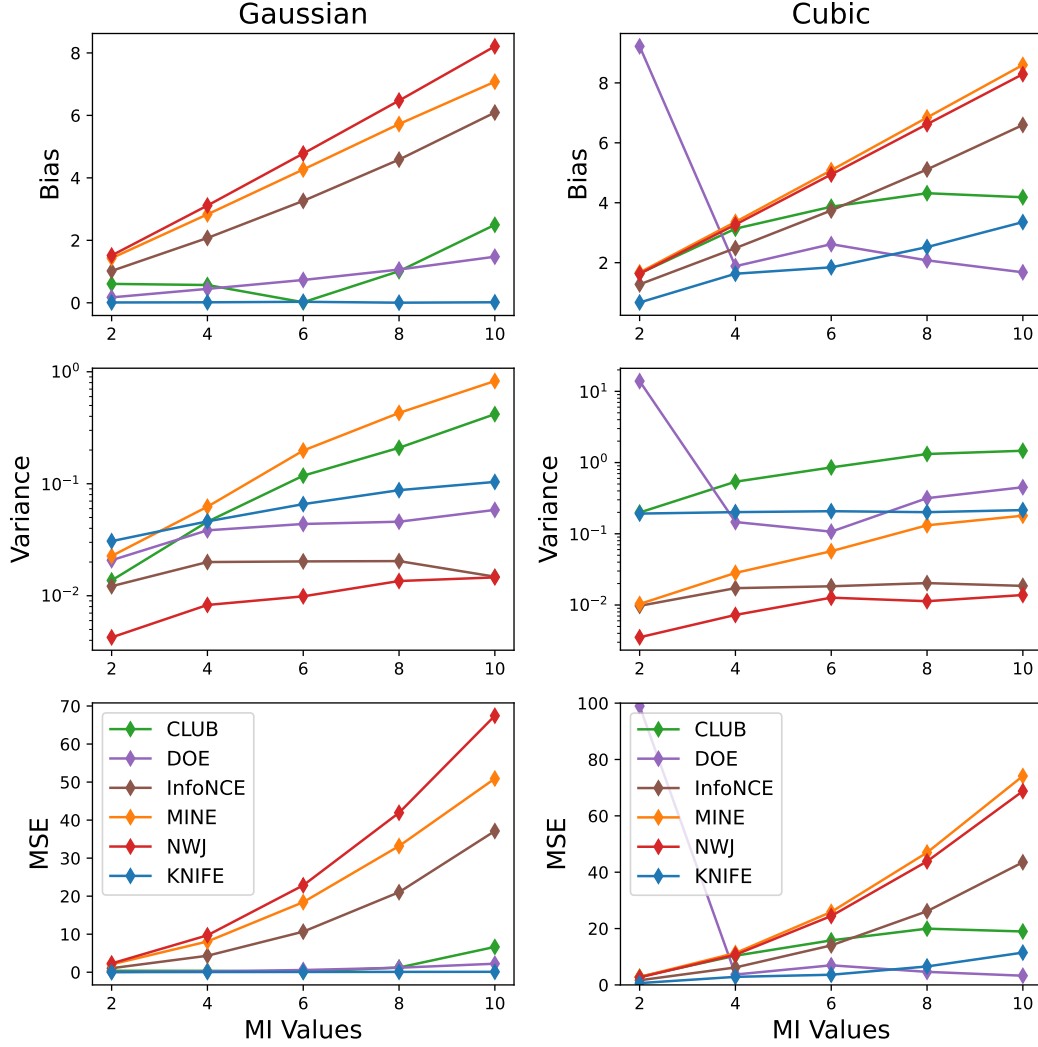

Figure 5: **Left:** Estimation of  $I(X; Y)$ ; **Right:** Estimation of  $I(X; Y^3)$  (cubic transformation).

574 **Computational Resources.** Training was performed, using about 6 hours of GPU time on an  
575 NVidia V100 GPU to carry out the experiment depicted in Figure 3 (bottom).

## 576 B Experimental Details of Experiments on Natural Data

### 577 B.1 Information Bottleneck for Language Model Finetuning

578 For this experiment we follow the experimental setting introduced in [27].<sup>4</sup>

579 **Model Architecture.** We report in Table 8, the multilayer perceptron (MLP) used to compute the  
580 compressed sentence representations produced by BERT. Variance and Mean MLP networks are  
581 composed of fully connected layers.

582 **Model Training.** For model training, all models are trained for 6 epochs and we use early stopping  
583 (best model is selected on validation set error). For IB,  $\lambda$  is selected in  $\{10^{-4}, 10^{-5}, 10^{-6}\}$  and  $K$  is  
584 selected in  $\{144, 192, 288, 384\}$ . We follow [29] where the posterior is averaged over 5 samples and  
585 a linear annealing schedule is used for  $\lambda$ . Additional hyper-parameters are reported in Table 9.

<sup>4</sup>We build on the code provided in <https://githubmemory.com/repo/rabeehk/vibert>.

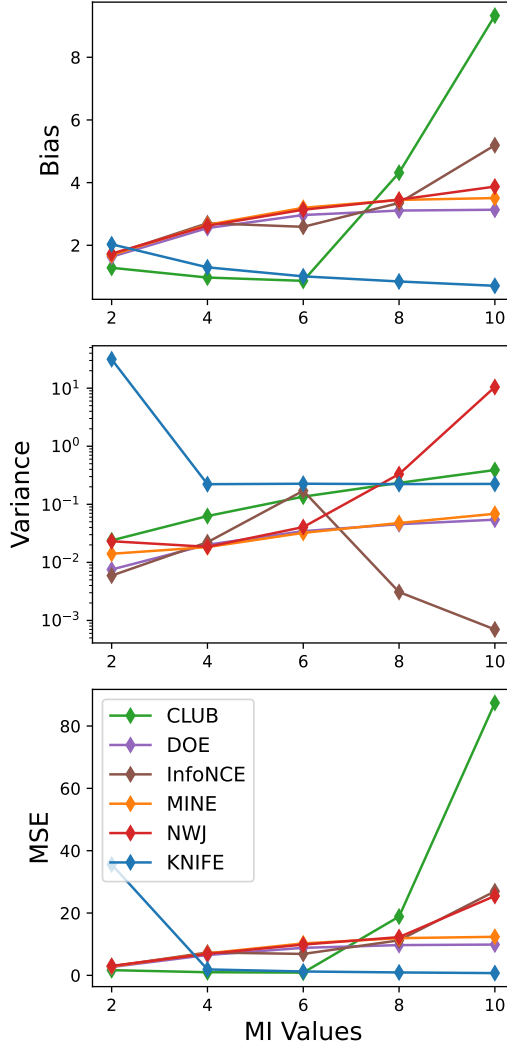

Figure 6: Bias, variance, and MSE for MI estimation on uniformly distributed data.

Table 8: Architecture of the model used in the IB finetuning experiment. We use ReLU as an activation function.

| Layer type      | Input shape        | Output shape       |
|-----------------|--------------------|--------------------|
| Fully connected | 768                | $\frac{2304+K}{4}$ |
| Fully connected | $\frac{2304+K}{4}$ | $\frac{768+K}{2}$  |

Table 9: Experimental details on Information Bottleneck.

| Parameter     | Value                              |
|---------------|------------------------------------|
| Learning Rate | See <a href="#">subsection B.1</a> |
| Optimizer     | AdamW                              |
| Warmup Steps  | 0.0                                |
| Dropout       | 0.0                                |
| Batch Size    | 32                                 |

Table 10: Datasets from the GLUE as used in our experiments.

|       | #Labels        | Train | Val.  | Test |
|-------|----------------|-------|-------|------|
| RTE   | 2              | 2.5k  | 0.08k | 3k   |
| STS-B | 1 (regression) | 5.8k  | 1.5k  | 1.4k |
| MRPC  | 2              | 3.7k  | 0.4k  | 1.7k |

586 **Dataset Statistics.** Table 10 reports the statistics of the dataset used in our finetuning experiment.

587 **Computational Resources.** For all these experiments we rely on NVidia-P100 with 16GB of RAM.  
 588 To complete the full grid-search on 10 seeds and on the three datasets, approximately 1.5k hours are  
 589 required.

## 590 B.2 Fair Textual Classification

591 In this section, we gather the experimental details for the textual fair classification task.

### 592 B.2.1 Details of the KNIFE-based Estimator

593 In this experiment, we estimate the MI between a continuous random variable, namely  $Z = \Phi_\psi(X)$ ,  
 594 and a discrete variable, denoted by  $S \in \mathcal{S} = \{1, 2, \dots, |\mathcal{S}|\}$ . We follow the strategy outlined in  
 595 Section 2.2 for estimating the conditional differential entropy  $h(Z|S)$ . However, we will reuse the  
 596 estimate of the conditional pdf  $\hat{p}(z|s; \Theta)$  to compute an estimate of the differential entropy as

$$h(Z) \approx -\frac{1}{N} \sum_{n=1}^N \log \left( \sum_{s \in \mathcal{S}} \hat{p}_{\text{KNIFE}}(z_n|s; \Theta) \hat{p}(s) \right), \quad (15)$$

597 where  $\hat{p}(s) = \frac{1}{N} |\{n : s_n = s\}|$  is used to indicate the empirical distribution of  $S$  in the training set  
 598  $\mathcal{D}_s$ .<sup>5</sup> In our experiments, with  $|\mathcal{S}| = 2$ , we found that estimating the differential entropy  $h(Z)$  based  
 599 on the KNIFE estimator learnt for  $h(Z|S)$  increases the stability of training.

### 600 B.2.2 Experimental Details

601 **Model Architecture.** For the encoder, we use a bidirectional GRU with two layers with hidden  
 602 and input dimension set to 128. We use LeakyReLU as the activation function. The classification  
 603 head is composed of fully connected layers of input dimension 256. We use a learning rate of 0.0001  
 604 for AdamW. The dropout rate is set to 0.2. The number of warmup steps is set to 1000.

605 **Computational Resources.** For all these experiments, we rely on NVIDIA-P100 with 16GB of  
 606 RAM. Each model is trained for 30k steps. The model with the lowest MI is selected. The training of  
 607 a single network takes around 3 hours.

## 608 B.3 Unsupervised Domain Adaptation

609 We follow the experimental setup given in [30] as closely as possible, i.e., we pick hyperparameters  
 610 given in the paper, or if not provided, those set in the code:<sup>6</sup>

611 **Model Training.** We use Adam optimizer for all modules with a learning rate of 0.001. Batch size  
 612 is set to 128. We set the weighting parameter  $\lambda = 0.1$ . The original code of [30] uses 15 000 training  
 613 iterations, but we found most methods had not properly converged at this stage, and hence use 25 000  
 614 iterations instead. Similar to other experiments, we set the kernel size  $M = 128$ .

615 **Model Architecture.** Table 11 summarizes the architectures used for the different modules. For  
 616 the MI network of each method, the best configuration, based on the validation set of the first task  
 617 MNIST  $\rightarrow$  MNIST-M, is chosen among 4 configurations: with or without LayerNorm and with ReLU  
 618 or tanh activation.

619 **Computational Resources.** For these experiments, we used a cluster of NVIDIA-V100 with 16GB  
 620 of RAM. Each training (i.e., 25k iterations) on a single task requires on average 2 hours. Given that  
 621 we have 6 tasks, and repeat the training for 3 different seeds, on average 36 hours computation time  
 622 is required for each method.

<sup>5</sup>As we work with balanced batches, we will have  $\hat{p}(s) = \frac{1}{|\mathcal{S}|}$ .

<sup>6</sup>[https://github.com/Linear95/CLUB/tree/master/MI\\_DA](https://github.com/Linear95/CLUB/tree/master/MI_DA).

Table 11: Architectures used for the Unsupervised Domain Adaptation experiments. For the MI network of each method, we chose the best performing configuration between with or without LayerNorm layer and best activation between ReLU and tanh, using the validation set of MNIST-M.

| <b>Encoder (both <math>\Phi</math> and <math>\Phi^d</math>)</b> |                      |                      |           |  |  |
|-----------------------------------------------------------------|----------------------|----------------------|-----------|--|--|
| Layer type                                                      | Input shape          | Output shape         | Details   |  |  |
| Convolution sequence                                            | (3, H, W)            | (64, H, W)           | Cf. below |  |  |
| Noisy downsampling                                              | (64, H, W)           | (64, H // 2, W // 2) | Cf. below |  |  |
| Convolution sequence                                            | (64, H // 2, W // 2) | (64, H // 2, W // 2) | Cf. below |  |  |
| Noisy downsampling                                              | (64, H // 2, W // 2) | (64, H // 4, W // 4) | Cf. below |  |  |
| Convolution sequence                                            | (64, H // 4, W // 4) | (64, H // 4, W // 4) | Cf. below |  |  |
| Global Average Pool                                             | (64, H // 4, W // 4) | (64,)                | -         |  |  |

  

| <b>Main classifier <math>C</math></b> |             |              | <b>Domain classifier <math>C^d</math></b> |             |              |
|---------------------------------------|-------------|--------------|-------------------------------------------|-------------|--------------|
| Layer type                            | Input shape | Output shape | Layer type                                | Input shape | Output shape |
| Fully connected                       | (64,)       | (10,)        | Fully connected                           | (64,)       | (2,)         |

  

| <b>Convolution sequence</b> |             |              |                                       |
|-----------------------------|-------------|--------------|---------------------------------------|
| Layer type                  | Input shape | Output shape | Parameters                            |
| 2D convolution              | (3, H, W)   | (64, H, W)   | 3x3, 64 channels, Stride=1, Padding=1 |
| 2D BatchNorm                | (3, H, W)   | (64, H, W)   | -                                     |
| Activation                  | (3, H, W)   | (64, H, W)   | LeakyRelu 0.1                         |
| 2D convolution              | (64, H, W)  | (64, H, W)   | 3x3, 64 channels, Stride=1, Padding=1 |
| 2D BatchNorm                | (64, H, W)  | (64, H, W)   | -                                     |
| Activation                  | (64, H, W)  | (64, H, W)   | LeakyRelu 0.1                         |
| 2D convolution              | (64, H, W)  | (64, H, W)   | 3x3, 64 channels, Stride=1, Padding=1 |
| 2D BatchNorm                | (64, H, W)  | (64, H, W)   | -                                     |
| Activation                  | (64, H, W)  | (64, H, W)   | LeakyRelu 0.1                         |

  

| <b>Noisy downsampling</b> |                      |                      |                            |
|---------------------------|----------------------|----------------------|----------------------------|
| Layer type                | Input shape          | Output shape         | Parameters                 |
| MaxPool                   | (64, H, W)           | (64, H // 2, H // 2) | 2x2, Stride=2              |
| Dropout                   | (64, H // 2, W // 2) | (64, H // 2, H // 2) | p=0.5                      |
| Noise                     | (64, H // 2, W // 2) | (64, H // 2, H // 2) | Gaussian with $\sigma = 1$ |

  

| <b>MI network</b> |               |                |                           |
|-------------------|---------------|----------------|---------------------------|
| Layer type        | Input shape   | Output shape   | Details                   |
| LayerNorm         | ( $C_{in,}$ ) | ( $C_{in,}$ )  | Optional                  |
| Fully connected   | ( $C_{in,}$ ) | (64,)          | Activation = [ReLU, tanh] |
| LayerNorm         | ( $C_{in,}$ ) | (64,)          |                           |
| Fully connected   | (64,)         | ( $C_{out,}$ ) | Optional                  |
